# Supplementary material for: Size and solvent effects on cellulose transverse anisotropy and toughening design
Source: arXiv:2606.05074 source file (2026-06-03)
Supplement: Supplementary file 1 [file cll_transverse_supplemenatary.tex]

\documentclass{article}
\usepackage{geometry}
\usepackage{graphicx}
\usepackage{hyperref}
\usepackage{subcaption}
\usepackage[numbers,comma,square,sort&compress]{natbib}
\geometry{a4paper,scale=0.9}
\graphicspath{{cll_transverse_images/}}
\linespread{1.0}
\bibliographystyle{unsrt}

\begin{document}

\begin{center}
\LARGE Size and solvent effects on cellulose transverse\\
anisotropy and toughening design\\
\end{center}

\begin{center}
\renewcommand{\thefootnote}{\fnsymbol{footnote}}
Xu Dong$^{1,}$\footnote{Corresponding author, Email: donx@zuaa.zju.edu.cn}\\
$^{1}$\textit{Department of Engineering Mechanics, Zhejiang University, Hangzhou 310027, China}
\end{center}

\begin{center}
Keywords: cellulose, anisotropy, hydrogen bonds, structure design, structure optimization
\end{center}

\setcounter{section}{0}
\setcounter{subsection}{0}

\setcounter{table}{0}
\setcounter{figure}{0}
\setcounter{equation}{0}

\renewcommand{\thesection}{S\arabic{section}}
\renewcommand{\thesubsection}{S\arabic{subsection}}

\renewcommand{\thetable}{S\arabic{table}}
\renewcommand{\thefigure}{S\arabic{figure}}
\renewcommand{\theequation}{S\arabic{equation}}

\section*{Supplementary Information}
\addtocounter{section}{1}
\setcounter{subsection}{0}
\addcontentsline{toc}{section}{\protect\numberline{}Supplementary Information}\indent

\subsection*{Models and relaxations of cellulose nanocrystals Type I}\indent
\addcontentsline{toc}{subsection}{\protect\numberline{}Models and relaxations of cellulose nanocrystals Type I}\indent

Referring to the transverse crystal lattice dimension data (a=0.778~nm, b=0.820~nm, c=1.038~nm) and the cellulose chain residue orientation (tg or gt type), the Type I CNCs models were constructed using chains of polymerization degree of 10 (Figure \ref{fig:cellulose_nanocrystal_structure_and_models}).
In Type I, all chains were composed of tg type residues.
According to the hydrogen bonding pattern, Type I has a specific orthogonal structure with three characteristic directions, along, perpendicular to, and slant to the hydrogen bonding layers.

\begin{figure}[htbp]
    \centering
    \scriptsize
    \begin{subfigure}[b]{0.24\textwidth}
        \centering
        \includegraphics[width=0.96\textwidth]{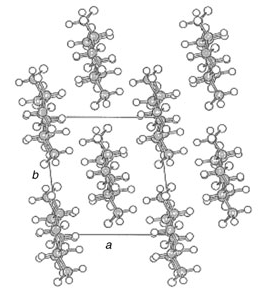}
        \subcaption{}
    \end{subfigure}
    \begin{subfigure}[b]{0.48\textwidth}
        \centering
        \includegraphics[width=0.96\textwidth]{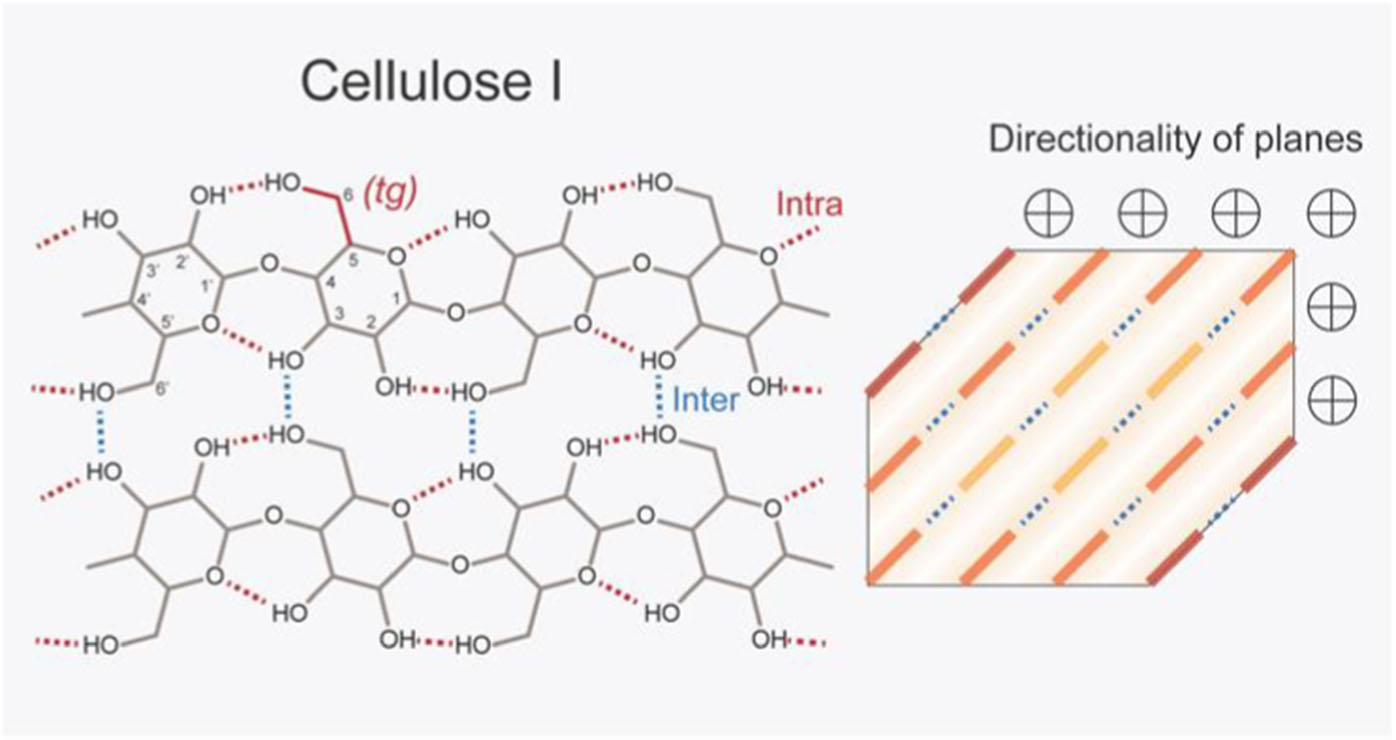}
        \subcaption{}
    \end{subfigure}
    \\
    \begin{subfigure}[b]{0.96\textwidth}
        \centering
        \includegraphics[width=0.96\textwidth]{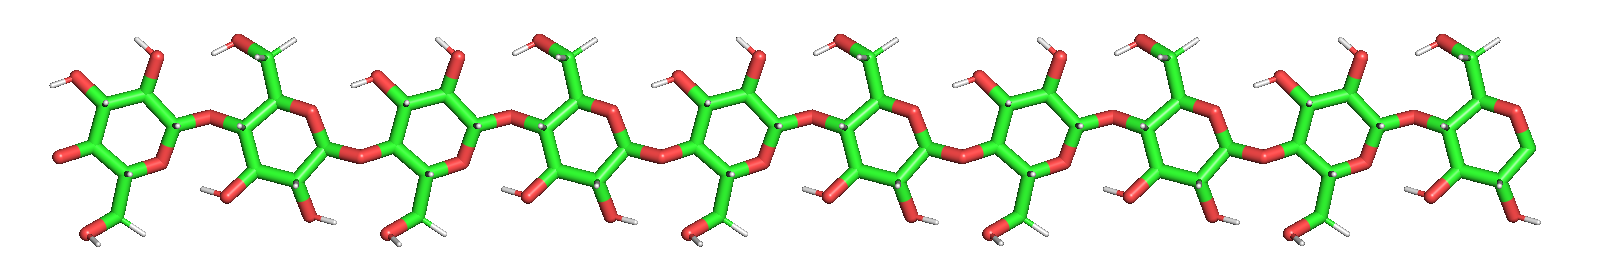}
        \subcaption{}
    \end{subfigure}
    \\
    \begin{subfigure}[b]{0.96\textwidth}
        \centering
        \begin{minipage}[b]{0.24\textwidth}
            \centering
            \includegraphics[width=0.96\textwidth]{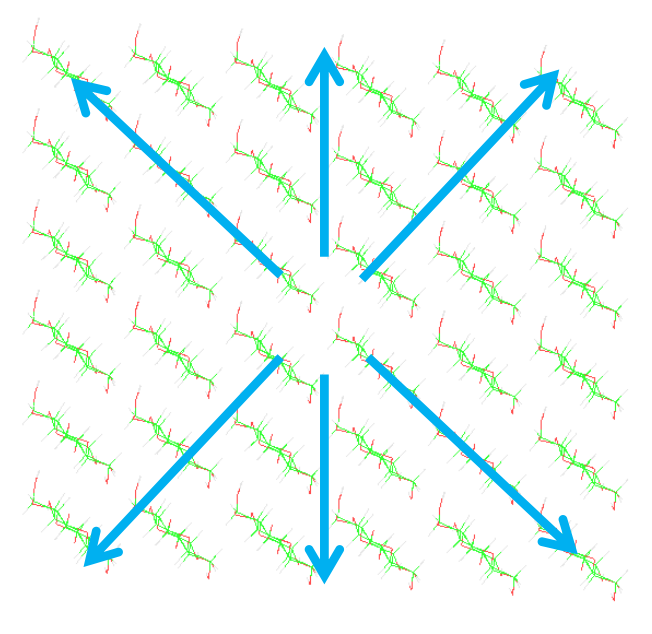}
        \end{minipage}
        \begin{minipage}[b]{0.20\textwidth}
            \centering
            \includegraphics[width=0.96\textwidth]{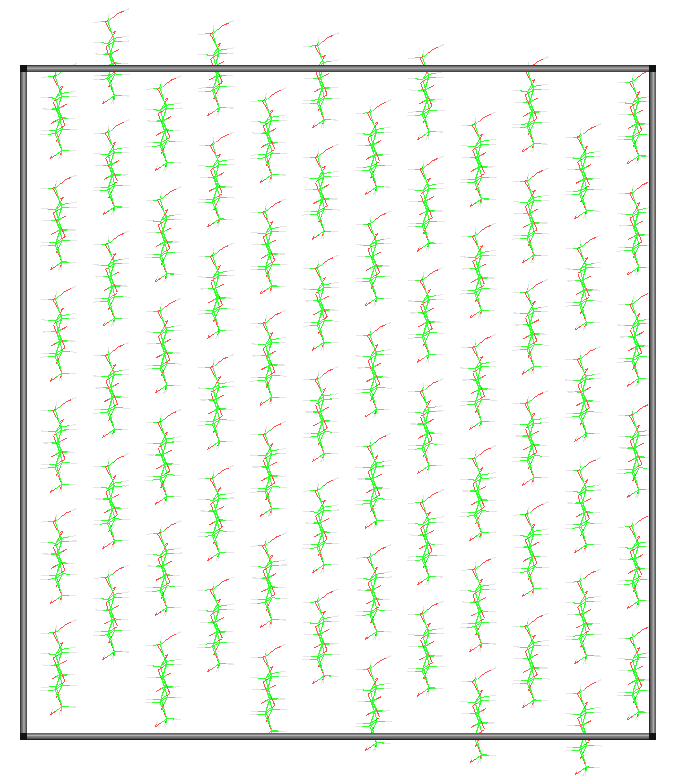}
            \\
            Vertical
        \end{minipage}
        \begin{minipage}[b]{0.255\textwidth}
            \centering
            \includegraphics[width=0.96\textwidth]{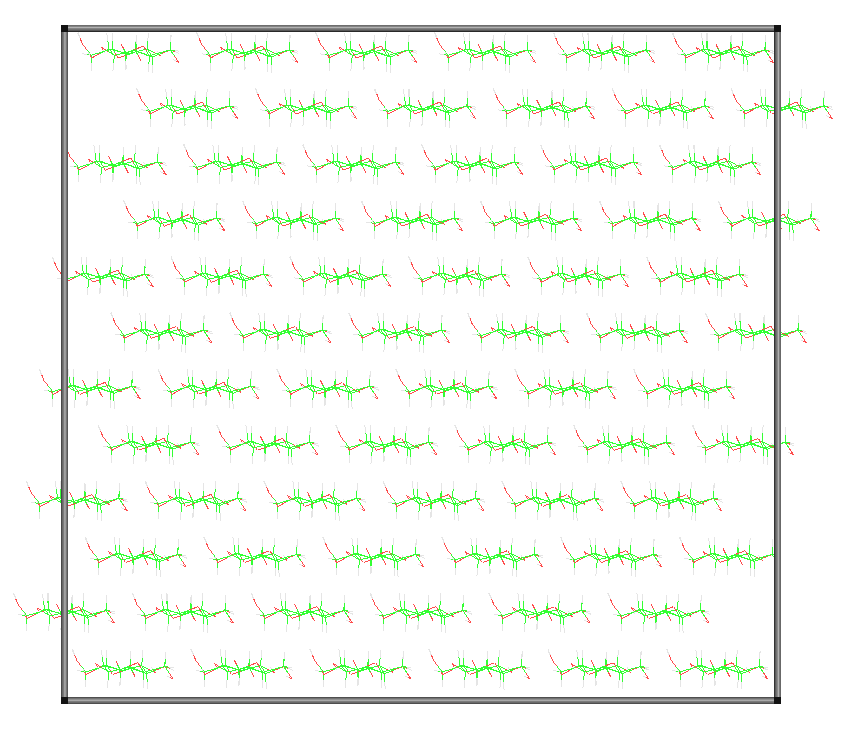}
            \\
            Horizontal
        \end{minipage}
        \begin{minipage}[b]{0.24\textwidth}
            \centering
            \includegraphics[width=0.96\textwidth]{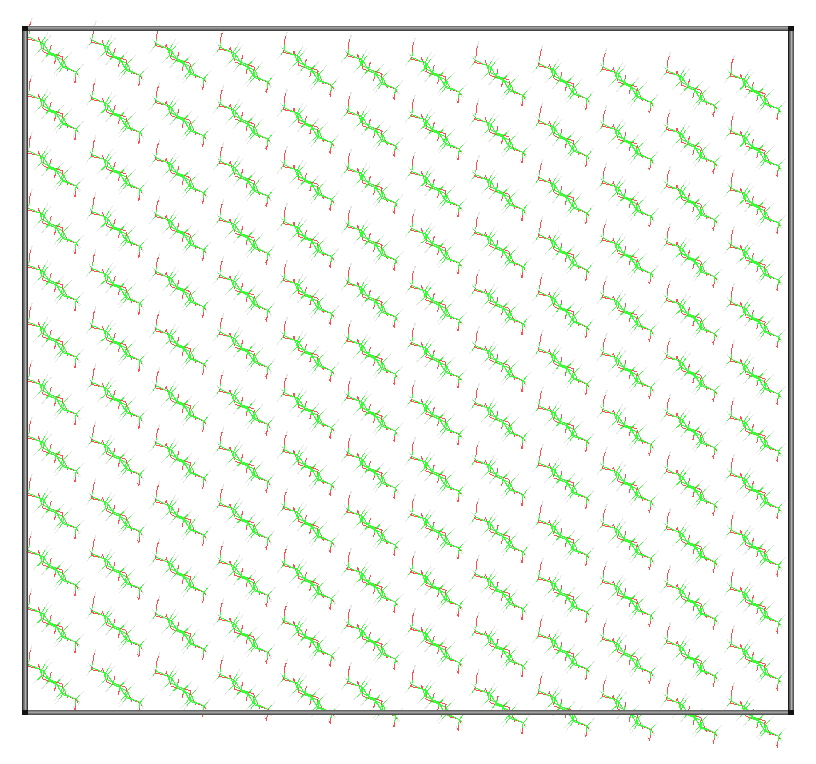}
            \\
            Slant
        \end{minipage}
        \subcaption{}
    \end{subfigure}
    \captionsetup{font=scriptsize}
    \caption{
    Structure and models of the Type I CNCs.
    (a) Lattice morphology and dimension.
    According to data provided in the literature, a=0.778~nm, b=0.820~nm, and axial c=1.038~nm.
    (b) Cross section and hydrogen bonding pattern.
    The Type I CNCs have a characteristic laminar structure dominated by hydrogen bonds.
    (c) Model of single periodic cellulose chain.
    The models for the three arrangement directions were composed of parallel periodic chains with a polymerization degree of 10, and each chain was alternately connected by residues.
    (d) Three characteristic directions of the Type I CNCs cross section and the corresponding three periodic models (vertical, horizontal, and slant arrangements).
    Considering the difficulty in applying shear loading in molecular dynamics, models with different arrangement directions were constructed and applied with the same vertical stretch loads.
    }
    \label{fig:cellulose_nanocrystal_structure_and_models}
\end{figure}

\clearpage

To fully examine the anisotropy in the cross section, vertical, horizontal, and slant models corresponding to characteristic directions were constructed using parallel chains, which bypassed the difficulty of applying shearing loads in molecular dynamics simulations.
For the slant model with inter layer frictional sliding, 144 chains were used, whereas the brittle vertical and horizontal models each contained 72 chains.
The structures after relaxation, and the RMSD curves of the models are shown in Figure \ref{fig:cellulose_nanocrystal_relaxations}.
These data demonstrate the stability of the Type I models and the relatively weak interactions between the inter hydrogen bonding layers.

\begin{figure}[htbp]
    \centering
    \scriptsize
    \begin{subfigure}[b]{0.96\textwidth}
        \centering
        \hspace{0.06\textwidth}
        \begin{minipage}[b]{0.20\textwidth}
            \centering
            \includegraphics[width=0.96\textwidth]{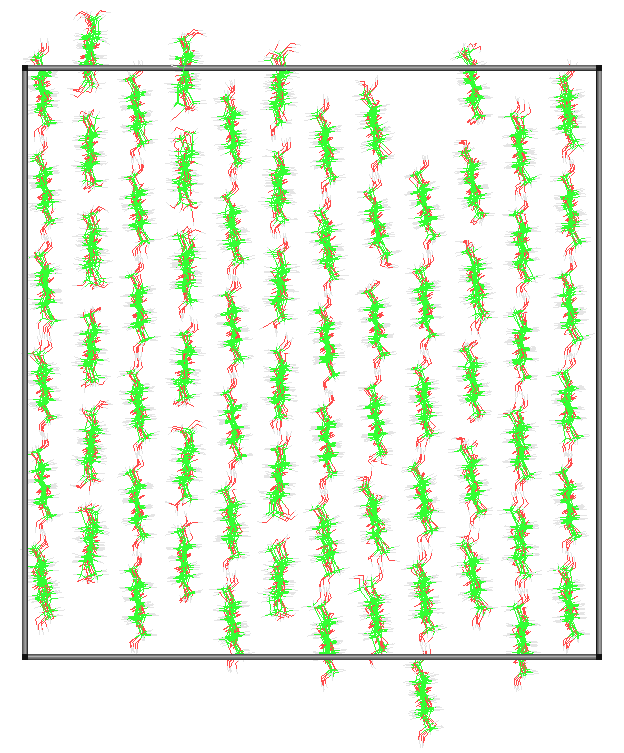}
        \end{minipage}
        \hspace{0.09\textwidth}
        \begin{minipage}[b]{0.255\textwidth}
            \centering
            \includegraphics[width=0.96\textwidth]{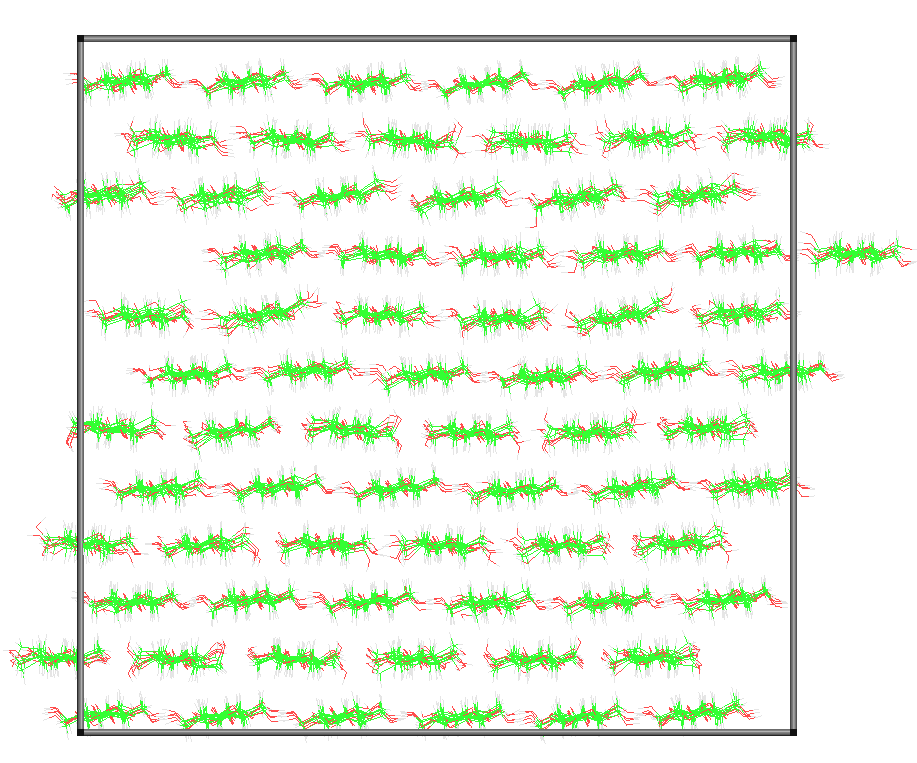}
        \end{minipage}
        \hspace{0.07\textwidth}
        \begin{minipage}[b]{0.24\textwidth}
            \centering
            \includegraphics[width=0.96\textwidth]{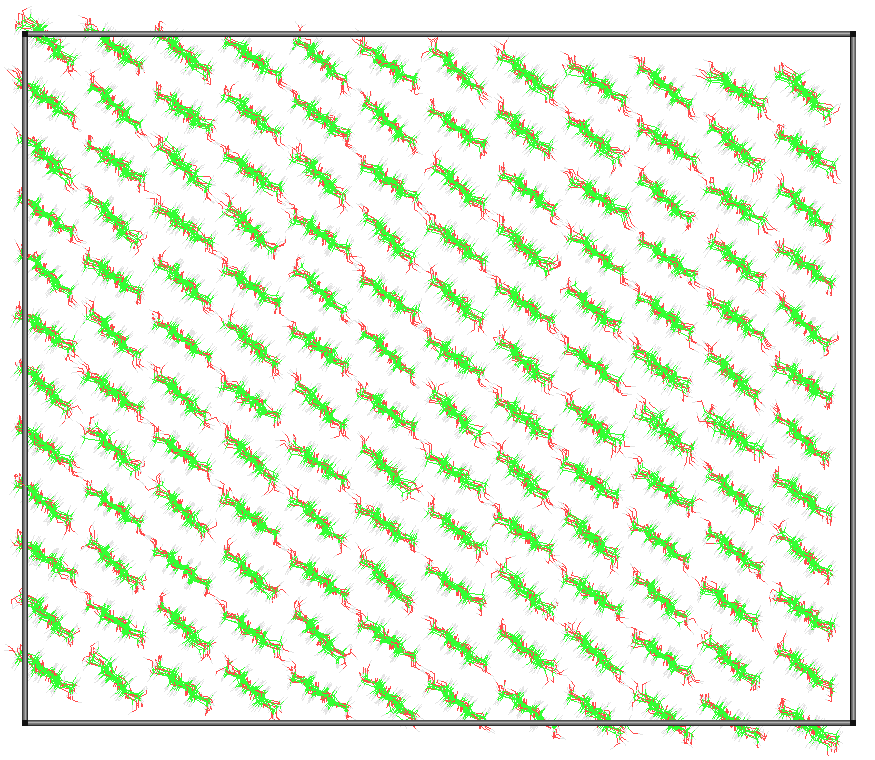}
        \end{minipage}
        \hspace{0.04\textwidth}
        \subcaption{}
    \end{subfigure}
    \\
    \begin{subfigure}[b]{0.96\textwidth}
        \centering
        \begin{minipage}[b]{0.32\textwidth}
            \centering
            \includegraphics[width=0.96\textwidth]{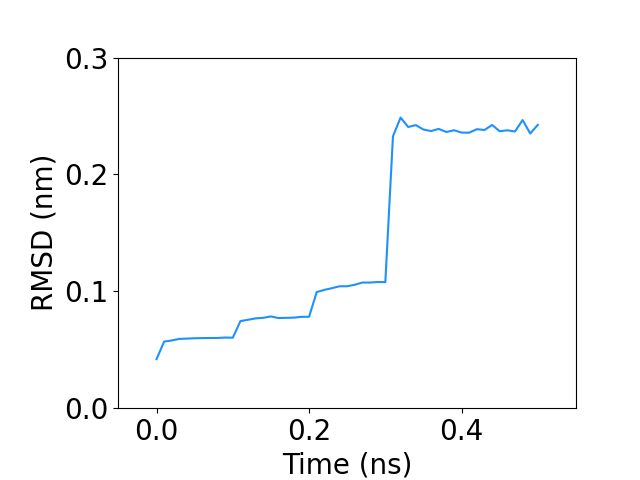}
            \\
            Vertical
        \end{minipage}
        \begin{minipage}[b]{0.32\textwidth}
            \centering
            \includegraphics[width=0.96\textwidth]{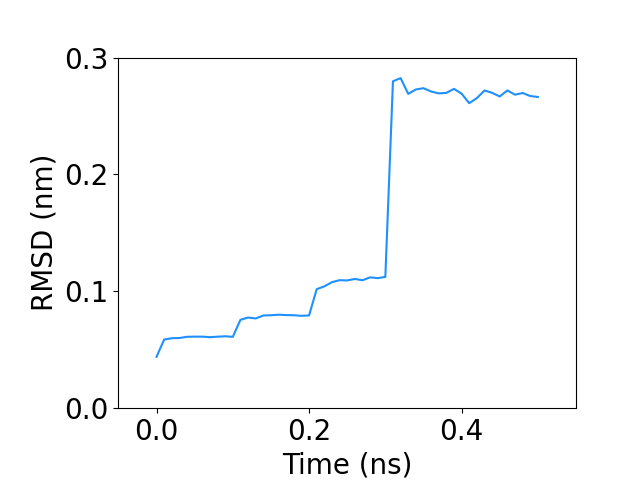}
            \\
            Horizontal
        \end{minipage}
        \begin{minipage}[b]{0.32\textwidth}
            \centering
            \includegraphics[width=0.96\textwidth]{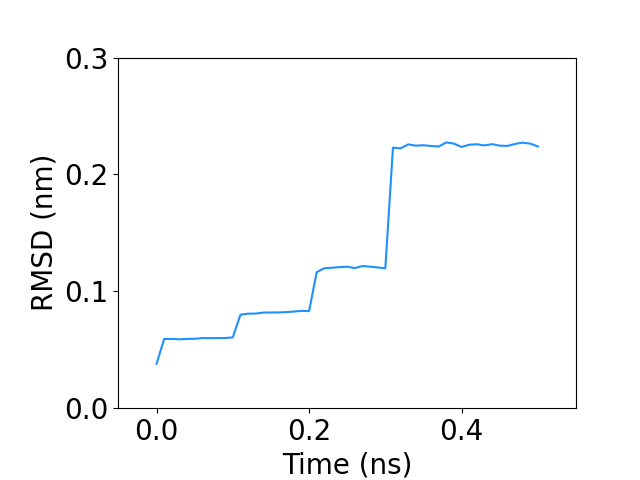}
            \\
            Slant
        \end{minipage}
        \subcaption{}
    \end{subfigure}
    \captionsetup{font=scriptsize}
    \caption{
    Relaxations of the Type I CNCs.
    (a) Structures of the vertical, horizontal, and slant models after energy minimization and relaxation.
    (b) RMSD curves during the relaxation process.
    The relaxation process imposed position constraints on the heavy atoms (carbon, oxygen, and nitrogen), which were gradually released in four stages.
    The structures after relaxation and the RMSD curves indicated no significant structural changes, with only layer sliding appearing in the vertical and horizontal models.
    }
    \label{fig:cellulose_nanocrystal_relaxations}
\end{figure}

\clearpage

\subsection*{Hydrogen bond number and potential energy during stretching of the Type I}\indent
\addcontentsline{toc}{subsection}{\protect\numberline{}Hydrogen bond number and potential energy during stretching of the Type I}\indent

The dominant role of hydrogen bonds and Coulomb interactions should be further elucidated, and the number of hydrogen bonds, and the Coulomb/van der Waals potential energies during stretching are shown in Figure \ref{fig:cellulose_nanocrystal_stretch_hydrogen_bond_number_and_energy}.
These data were all delta, indicating that they were relative to their corresponding minimum values, which also effectively set the zero potential energy surface.
The vertical model with the highest strength was the only case in which the Coulomb potential increased, thus emphasizing the dominant role of hydrogen bonds in this characteristic direction.
In addition, the greatest reduction in the hydrogen bond number in the vertical model also supported this, whereas the slant model partially recovered the hydrogen bond number after inter layer frictional sliding.
However, the van der Waals potential energy increased after stretching, indicating the general resistance of van der Waals interactions against external loads.

\begin{figure}[htbp]
    \centering
    \scriptsize
    \begin{subfigure}[b]{0.96\textwidth}
        \centering
        \begin{minipage}[b]{0.32\textwidth}
            \centering
            \includegraphics[width=0.96\textwidth]{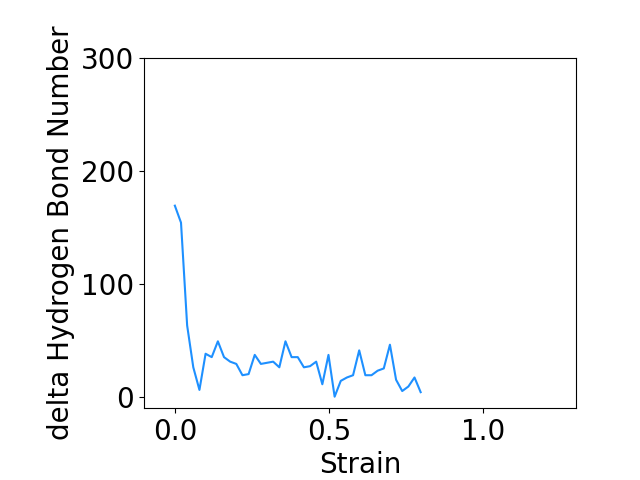}
        \end{minipage}
        \begin{minipage}[b]{0.32\textwidth}
            \centering
            \includegraphics[width=0.96\textwidth]{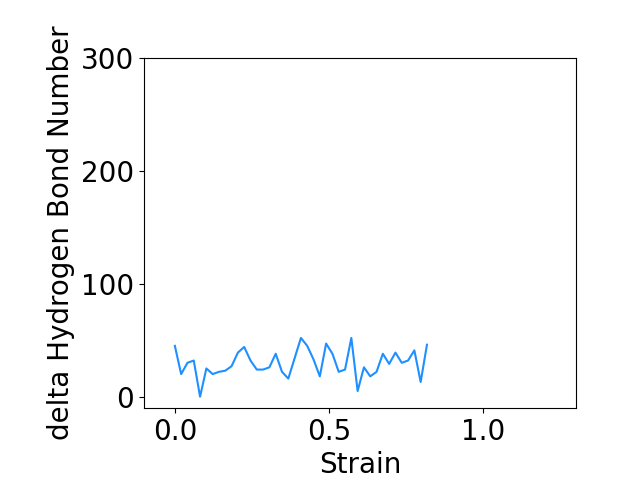}
        \end{minipage}
        \begin{minipage}[b]{0.32\textwidth}
            \centering
            \includegraphics[width=0.96\textwidth]{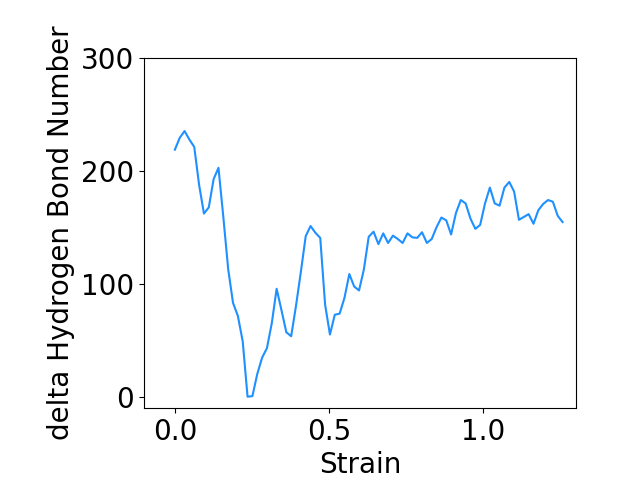}
        \end{minipage}
        \subcaption{}
    \end{subfigure}
    \\
    \begin{subfigure}[b]{0.96\textwidth}
        \centering
        \begin{minipage}[b]{0.32\textwidth}
            \centering
            \includegraphics[width=0.96\textwidth]{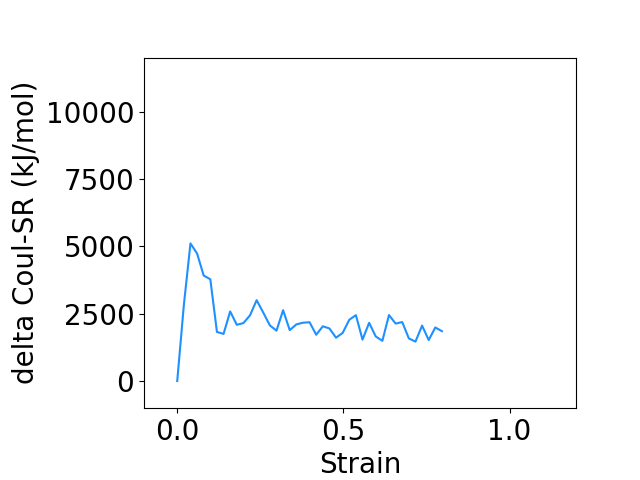}
        \end{minipage}
        \begin{minipage}[b]{0.32\textwidth}
            \centering
            \includegraphics[width=0.96\textwidth]{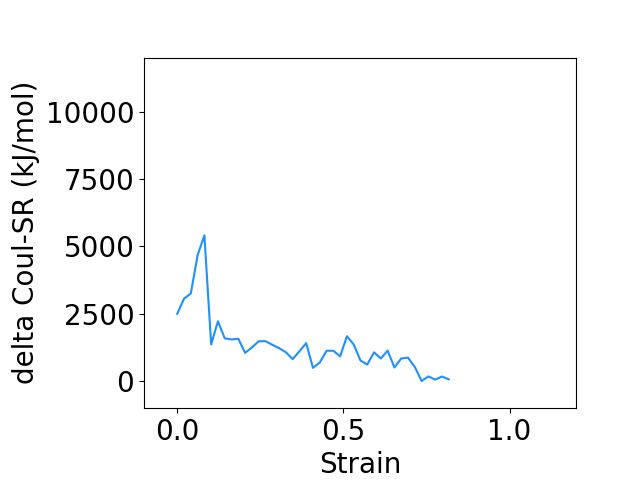}
        \end{minipage}
        \begin{minipage}[b]{0.32\textwidth}
            \centering
            \includegraphics[width=0.96\textwidth]{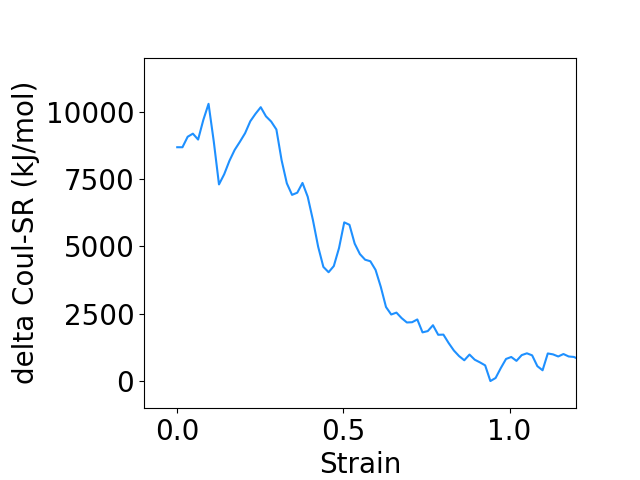}
        \end{minipage}
        \subcaption{}
    \end{subfigure}
    \\
    \begin{subfigure}[b]{0.96\textwidth}
        \centering
        \begin{minipage}[b]{0.32\textwidth}
            \centering
            \includegraphics[width=0.96\textwidth]{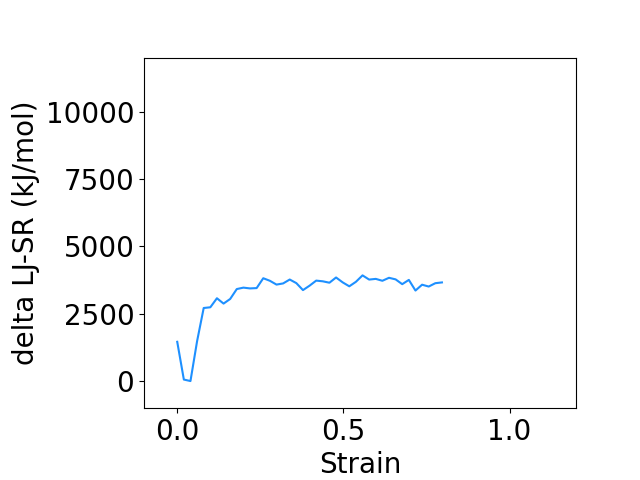}
            \\
            Vertical
        \end{minipage}
        \begin{minipage}[b]{0.32\textwidth}
            \centering
            \includegraphics[width=0.96\textwidth]{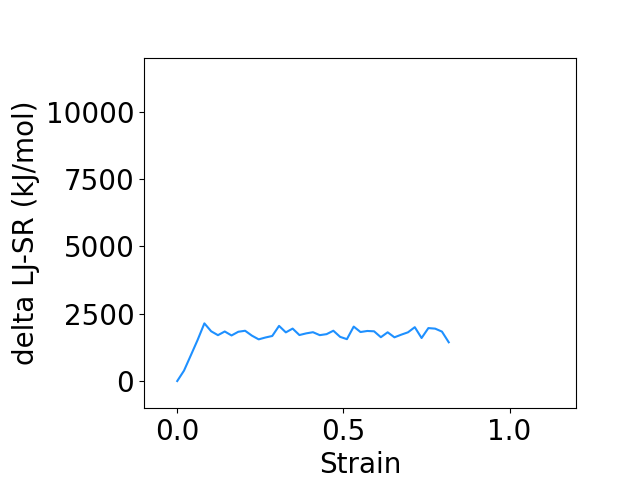}
            \\
            Horizontal
        \end{minipage}
        \begin{minipage}[b]{0.32\textwidth}
            \centering
            \includegraphics[width=0.96\textwidth]{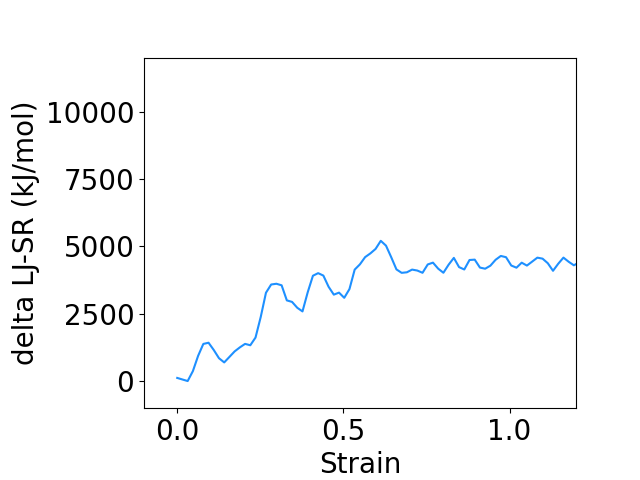}
            \\
            Slant
        \end{minipage}
        \subcaption{}
    \end{subfigure}
    \captionsetup{font=scriptsize}
    \caption{
    Hydrogen bond number and potential energy curves during stretching of the Type I CNCs.
    (a) Number of hydrogen bonds during stretching.
    Hydrogen bonds played a vital role in the high strength of the vertical model and decreased the most.
    For the slant model with inter layer frictional sliding, the hydrogen bond number recovered after fracture.
    (b) Coulomb potential energy and (c) van der Waals potential energy curves during stretching of the vertical, horizontal, and slant models.
    The curves shown are relative to their respective minimum values; effectively, the zero potential energy surface was set to the lowest potential energy value.
    During the stretching of the vertical model, the Coulomb potential energy increased whereas it decreased in the other models, corresponding to the dominant role of hydrogen bonding in the vertical arrangement.
    Although the van der Waals potential energy increased in all three models, the magnitude of the increase followed the order (slant \textgreater vertical \textgreater horizontal), corresponding to the inter layer frictional sliding phenomenon in the slant model.
    These comprehensive analyses showed that even in the vertical model where Coulomb interaction dominates, the contribution of van der Waals interactions to the strain energy remains important.
    }
    \label{fig:cellulose_nanocrystal_stretch_hydrogen_bond_number_and_energy}
\end{figure}

\clearpage

\subsection*{Models and relaxations of cellulose nanocrystals Type II}\indent
\addcontentsline{toc}{subsection}{\protect\numberline{}Models and relaxations of cellulose nanocrystals Type II}\indent

Referring to the transverse crystal lattice dimension data (a=0.810~nm, b=0.903~nm, and c=1.031~nm) and the cellulose chain residue orientation (tg or gt type), the Type II CNCs models were constructed using chains of polymerization degree of 10 (Figure \ref{fig:cellulose_nanocrystal_ii_structure_and_models}).
In Type II, all chains were composed of alternate tg and gt type residues.
According to the hydrogen bonding pattern, Type II has a laminar structure with two characteristic directions.
For Type II, the characteristic directions were selected based on the directions of the crystal lattice. 

\begin{figure}[htbp]
    \centering
    \scriptsize
    \begin{subfigure}[b]{0.32\textwidth}
        \centering
        \includegraphics[width=0.96\textwidth]{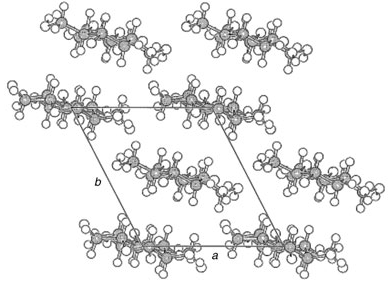}
        \subcaption{}
    \end{subfigure}
    \begin{subfigure}[b]{0.48\textwidth}
        \centering
        \includegraphics[width=0.96\textwidth]{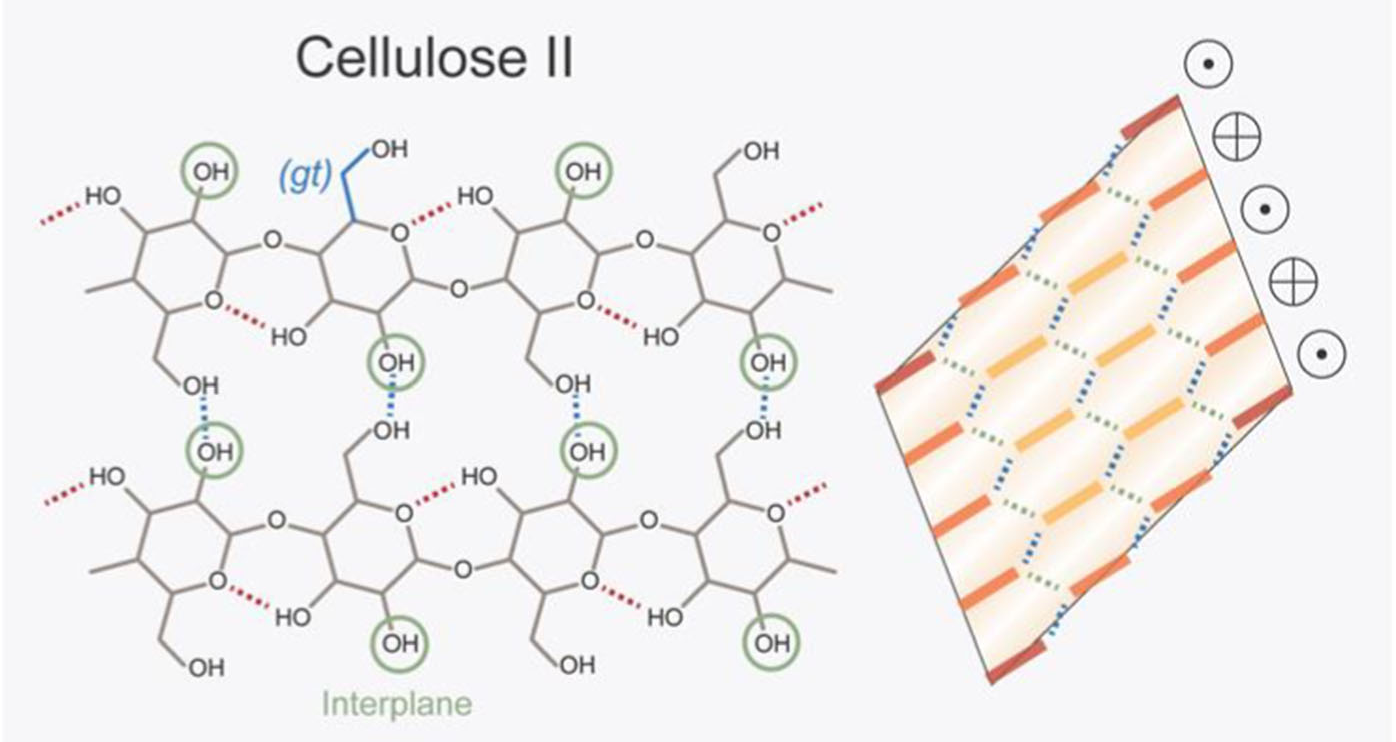}
        \subcaption{}
    \end{subfigure}
    \\
    \begin{subfigure}[b]{0.96\textwidth}
        \centering
        \includegraphics[width=0.96\textwidth]{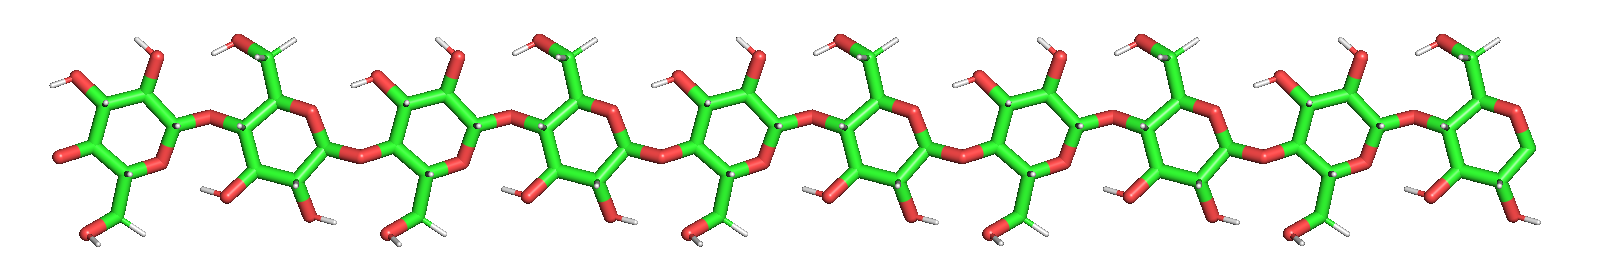}
        \\
        \includegraphics[width=0.96\textwidth]{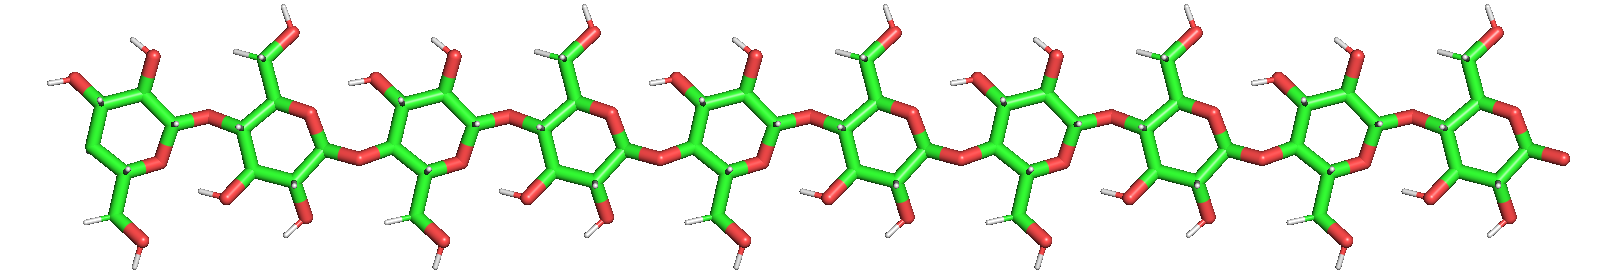}
        \subcaption{}
    \end{subfigure}
    \\
    \begin{subfigure}[b]{0.96\textwidth}
        \centering
        \begin{minipage}[b]{0.24\textwidth}
            \centering
            \includegraphics[width=0.96\textwidth]{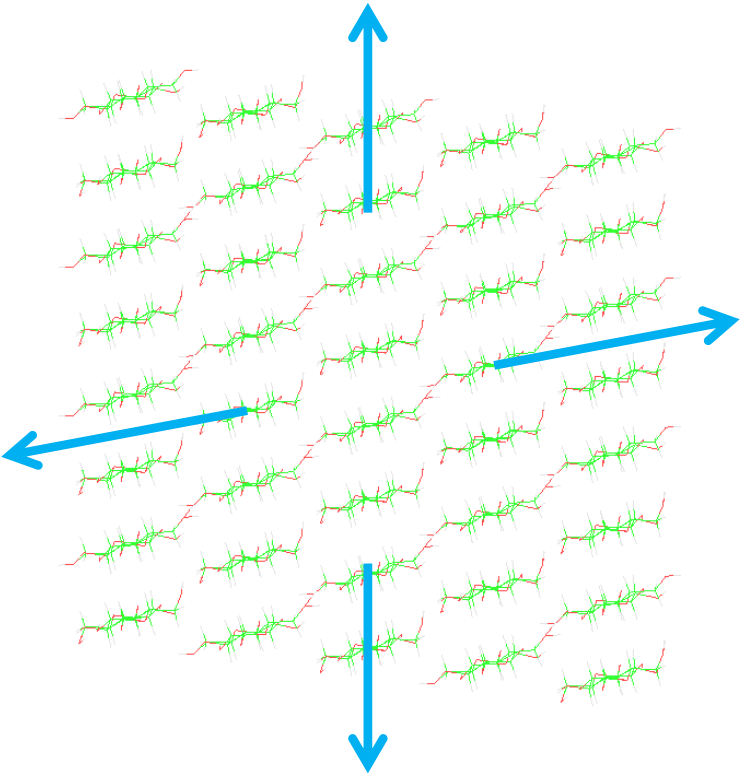}
        \end{minipage}
        \begin{minipage}[b]{0.24\textwidth}
            \centering
            \includegraphics[width=0.96\textwidth]{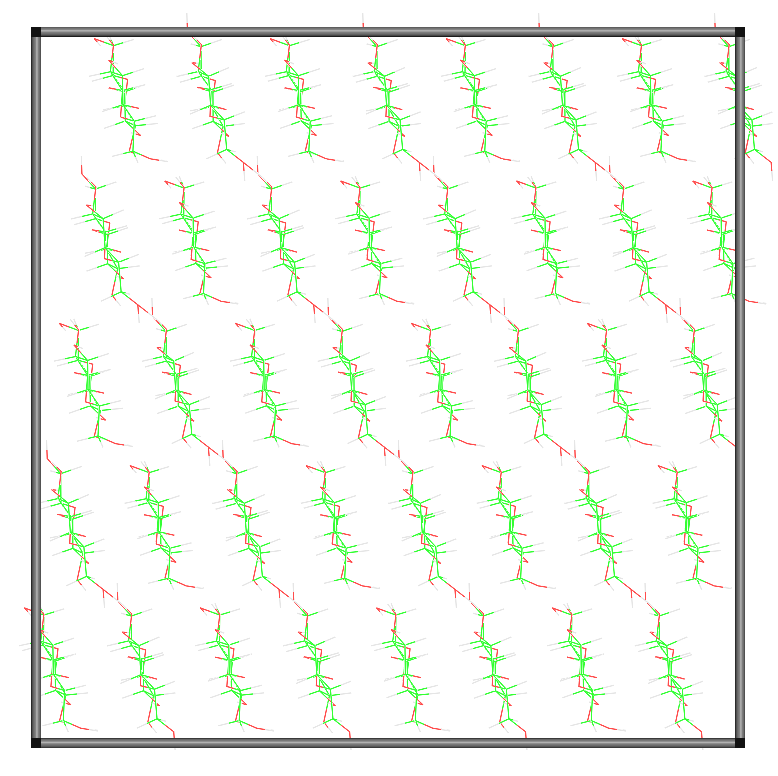}
            \\
            Vertical
        \end{minipage}
        \begin{minipage}[b]{0.24\textwidth}
            \centering
            \includegraphics[width=0.96\textwidth]{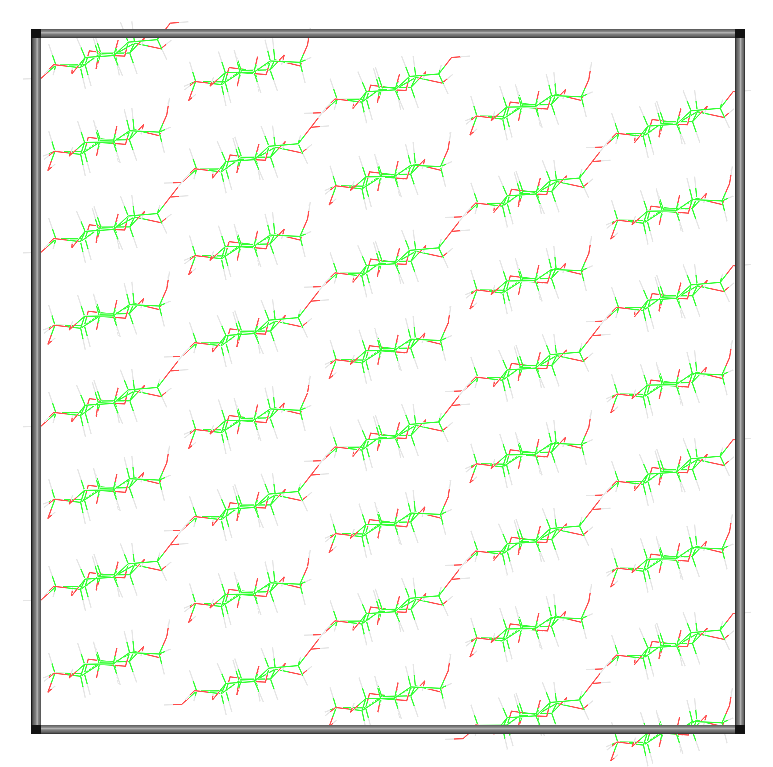}
            \\
            Slant
        \end{minipage}
        \subcaption{}
    \end{subfigure}
    \captionsetup{font=scriptsize}
    \caption{
    Structure and models of the Type II CNCs.
    (a) Lattice morphology and dimension.
    According to the information provided in the literature, a=0.810~nm, b=0.903~nm, and axial c=1.031~nm.
    (b) Cross section and hydrogen bonding pattern.
    Type II CNCs exhibits a characteristic laminar structure dominated by hydrogen bonds.
    (c) Models of two type single periodic cellulose chains.
    The models for the two arrangement directions were composed of parallel periodic chains with a polymerization degree of 10, and each chain was alternately connected by residues.
    In contrast, Type II was composed of two types of chains with different side chain orientations;
    the tg type was the same as that in Type I, while the other gt type had the opposite side chain orientation.
    The gt type stresses inter chain hydrogen bonds more and provides fewer intra chain hydrogen bonds.
    (d) Two characteristic directions of the Type II CNCs cross section and the corresponding two periodic models (vertical, and slant arrangements).
    These characteristic directions corresponded to the directions of the crystal lattice.
    Considering the difficulty in applying shear loading in molecular dynamics, models with different arrangement directions were constructed and applied with the same vertical stretch loads.
    }
    \label{fig:cellulose_nanocrystal_ii_structure_and_models}
\end{figure}

\clearpage

To fully examine the anisotropy in the cross section, vertical and slant models corresponding to characteristic directions were constructed using parallel chains, which bypassed the difficulty of applying shearing loads in molecular dynamics simulations.
Both the vertical and slant models contained 40 chains.
The structures after relaxation, and the RMSD curves of the models are shown in Figure \ref{fig:cellulose_nanocrystal_ii_relaxations}.
These data indicate the stability of the Type II models, which was better than that of the Type I models, as shown by the RMSD curves.

\begin{figure}[htbp]
    \centering
    \scriptsize
    \begin{subfigure}[b]{0.96\textwidth}
        \centering
        \hspace{0.04\textwidth}
        \begin{minipage}[b]{0.24\textwidth}
            \centering
            \includegraphics[width=0.96\textwidth]{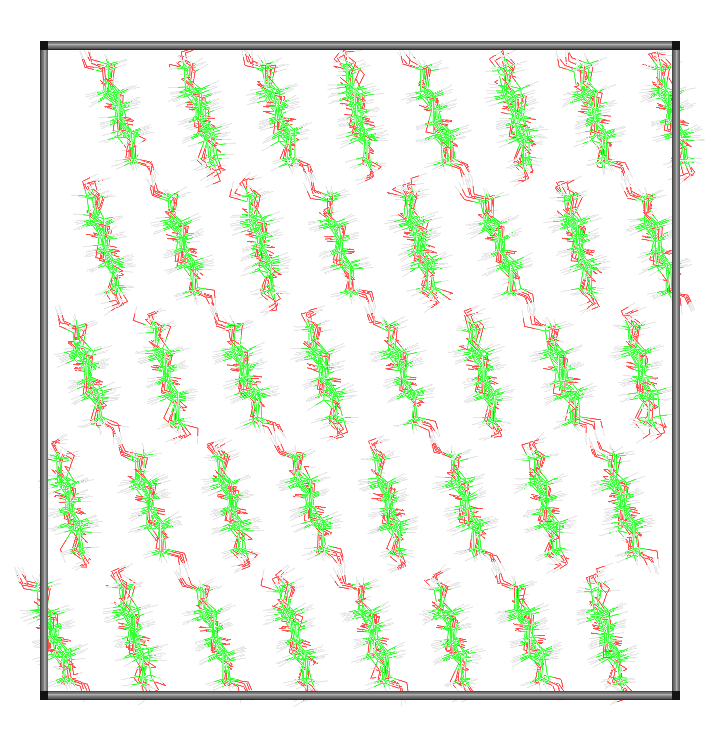}
        \end{minipage}
        \hspace{0.08\textwidth}
        \begin{minipage}[b]{0.24\textwidth}
            \centering
            \includegraphics[width=0.96\textwidth]{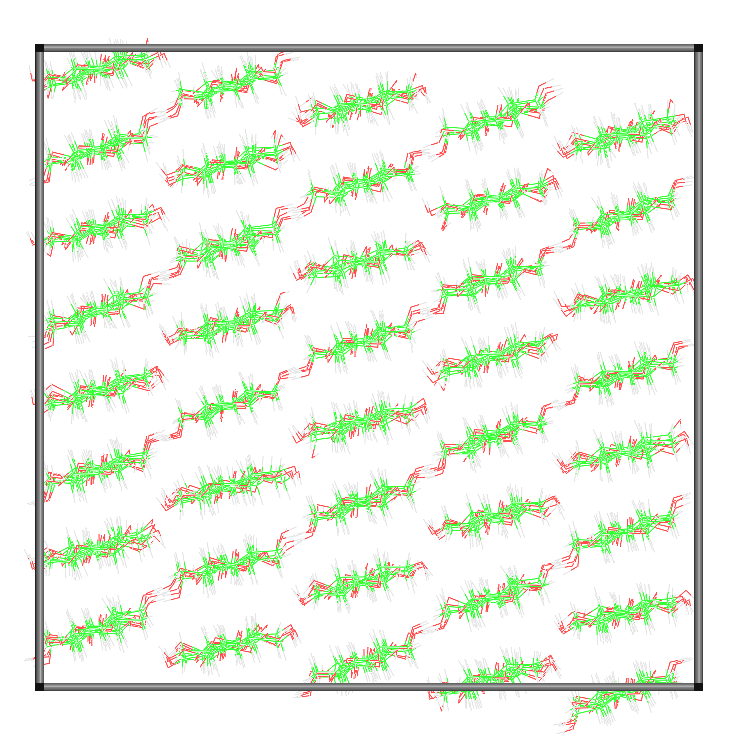}
        \end{minipage}
        \hspace{0.36\textwidth}
        \subcaption{}
    \end{subfigure}
    \\
    \begin{subfigure}[b]{0.96\textwidth}
        \centering
        \begin{minipage}[b]{0.32\textwidth}
            \centering
            \includegraphics[width=0.96\textwidth]{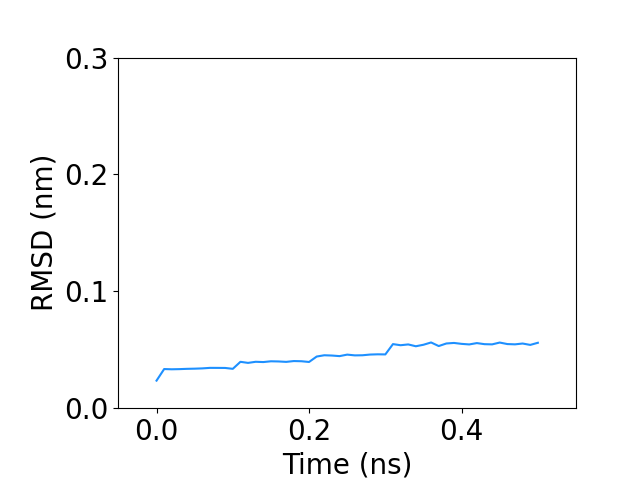}
            \\
            Vertical
        \end{minipage}
        \begin{minipage}[b]{0.32\textwidth}
            \centering
            \includegraphics[width=0.96\textwidth]{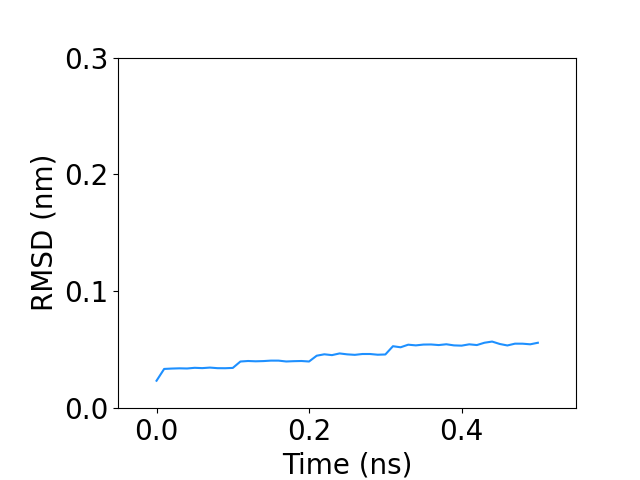}
            \\
            Slant
        \end{minipage}
        \begin{minipage}[b]{0.32\textwidth}
            \centering
            \includegraphics[width=0.96\textwidth]{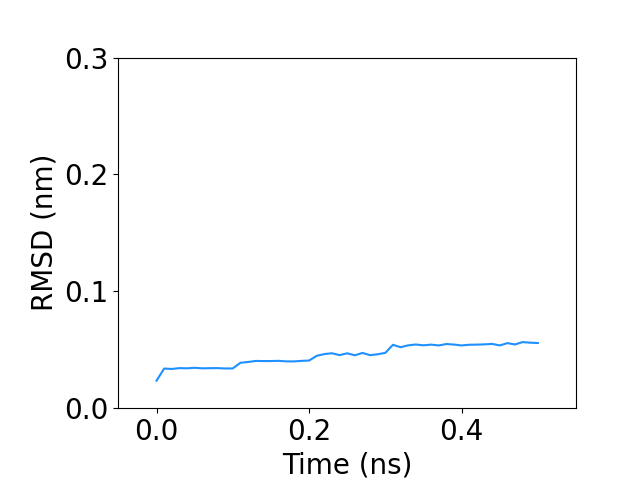}
            \\
            Slant Tough
        \end{minipage}
        \subcaption{}
    \end{subfigure}
    \captionsetup{font=scriptsize}
    \caption{
    Relaxations of the Type II CNCs.
    (a) Structures of the vertical and slant models after energy minimization and relaxation.
    (b) RMSD curves during the relaxation process.
    The relaxation process imposed position constraints on the heavy atoms (carbon, oxygen, and nitrogen), which were gradually released in four stages.
    The structures after relaxation and the RMSD curves indicated no significant structural changes, and is more stable if compared with Type I.
    }
    \label{fig:cellulose_nanocrystal_ii_relaxations}
\end{figure}

\clearpage

\subsection*{Hydrogen bond number and potential energy during stretching of the Type II}\indent
\addcontentsline{toc}{subsection}{\protect\numberline{}Hydrogen bond number and potential energy during stretching of the Type II}\indent

The dominant role of hydrogen bonds and Coulomb interactions should be further elucidated, and the number of hydrogen bonds, and the Coulomb/van der Waals potential energies during stretching are shown in Figure \ref{fig:cellulose_nanocrystal_ii_stretch_hydrogen_bond_number_and_energy}.
These data were all delta, indicating that they were relative to their corresponding minimum values, which also effectively set the zero potential energy surface.
Considering the important restructuring phenomenon of the slant model, the ``Slant Tough'' data corresponding to the restructuring are presented.
The vertical model with the highest strength had the steepest curves of the hydrogen bond number and Coulomb potential energy, stressing the crucial role of hydrogen bonds.
In contrast to laminar Type I with inter layer frictional sliding, the structure of Type II is significantly stiffer, and all the potential energy curves increased during stretching.
Therefore, both the Coulomb and van der Waals interactions are important for resisting external loads in Type II.

\begin{figure}[htbp]
    \centering
    \scriptsize
    \begin{subfigure}[b]{0.96\textwidth}
        \centering
        \begin{minipage}[b]{0.32\textwidth}
            \centering
            \includegraphics[width=0.96\textwidth]{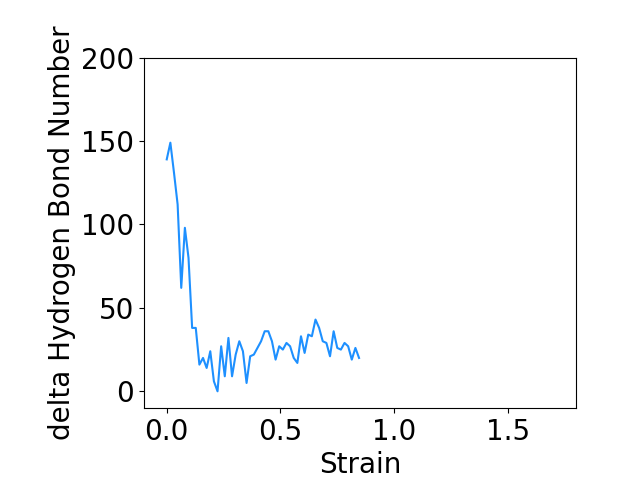}
        \end{minipage}
        \begin{minipage}[b]{0.32\textwidth}
            \centering
            \includegraphics[width=0.96\textwidth]{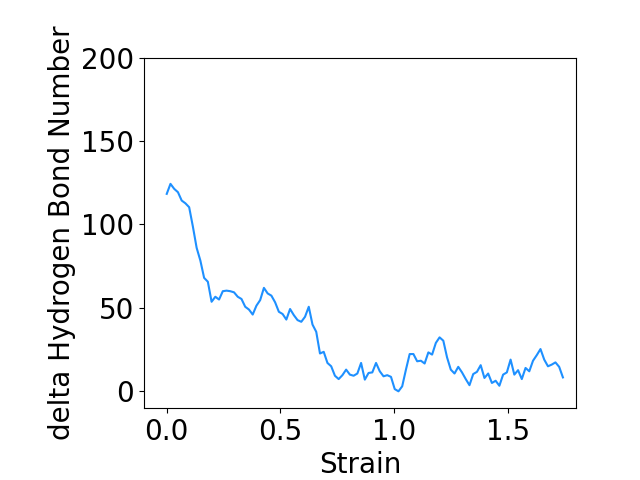}
        \end{minipage}
        \begin{minipage}[b]{0.32\textwidth}
            \centering
            \includegraphics[width=0.96\textwidth]{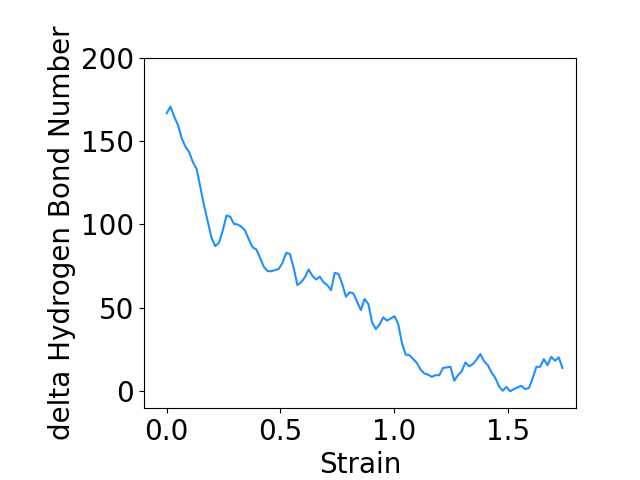}
        \end{minipage}
        \subcaption{}
    \end{subfigure}
    \\
    \begin{subfigure}[b]{0.96\textwidth}
        \centering
        \begin{minipage}[b]{0.32\textwidth}
            \centering
            \includegraphics[width=0.96\textwidth]{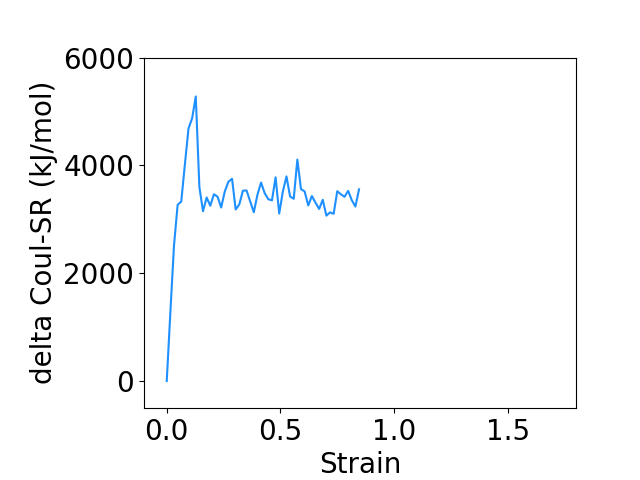}
        \end{minipage}
        \begin{minipage}[b]{0.32\textwidth}
            \centering
            \includegraphics[width=0.96\textwidth]{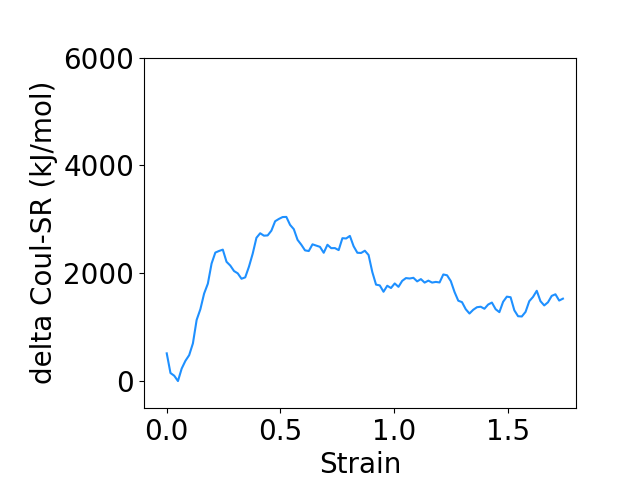}
        \end{minipage}
        \begin{minipage}[b]{0.32\textwidth}
            \centering
            \includegraphics[width=0.96\textwidth]{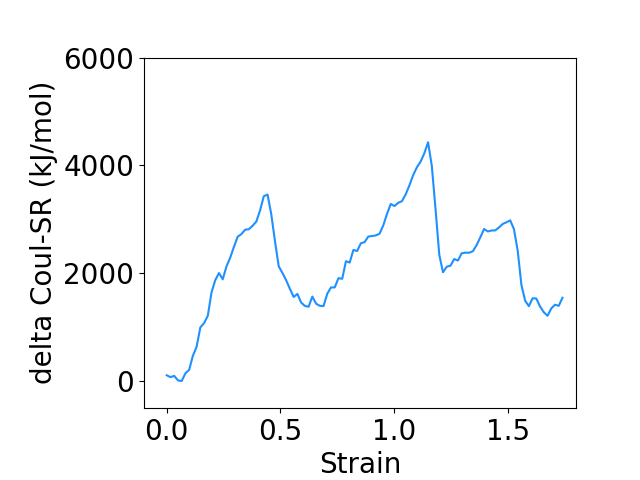}
        \end{minipage}
        \subcaption{}
    \end{subfigure}
    \\
    \begin{subfigure}[b]{0.96\textwidth}
        \centering
        \begin{minipage}[b]{0.32\textwidth}
            \centering
            \includegraphics[width=0.96\textwidth]{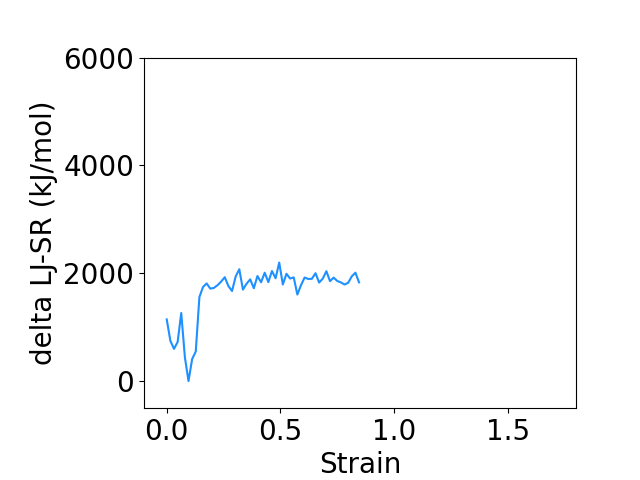}
            \\
            Vertical
        \end{minipage}
        \begin{minipage}[b]{0.32\textwidth}
            \centering
            \includegraphics[width=0.96\textwidth]{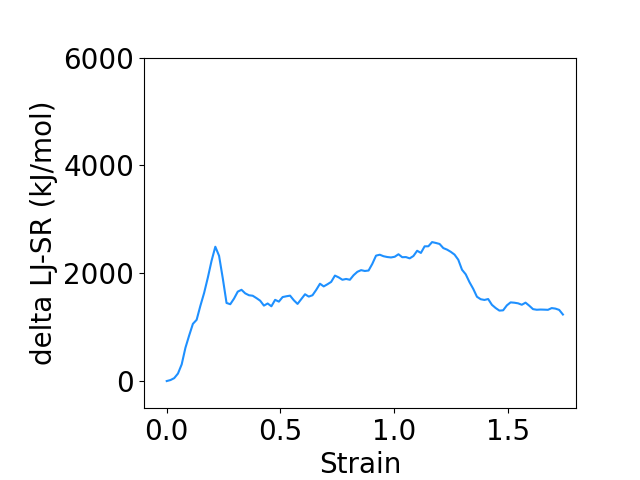}
            \\
            Slant
        \end{minipage}
        \begin{minipage}[b]{0.32\textwidth}
            \centering
            \includegraphics[width=0.96\textwidth]{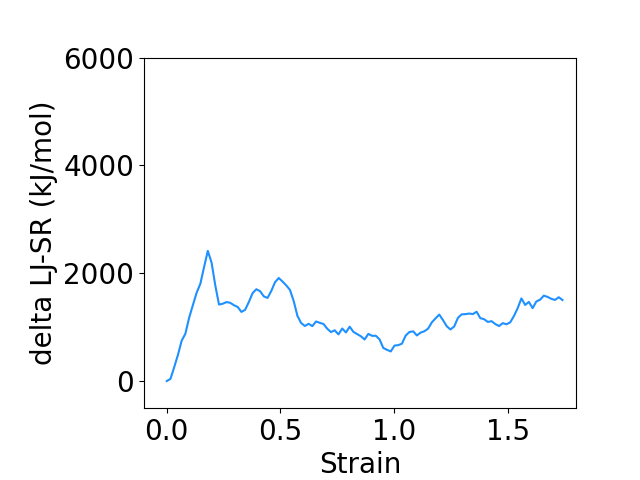}
            \\
            Slant Tough
        \end{minipage}
        \subcaption{}
    \end{subfigure}
    \captionsetup{font=scriptsize}
    \caption{
    Hydrogen bond number and potential energy curves during stretching of the Type II CNCs.
    (a) Number of hydrogen bonds during stretching.
    The fractures of both models involved the breaking of hydrogen bonds, but the curve of the vertical model was the steepest.
    (b) Coulomb potential energy and (c) van der Waals potential energy curves during stretching of the vertical, horizontal, and slant models.
    The curves shown are relative to their respective minimum values; effectively, the zero potential energy surface was set to the lowest potential energy value.
    Considering the possible restructuring with higher toughness of the slant model, the ``Slant Tough'' case with a restructuring was also included.
    During the stretching of the vertical model, the Coulomb potential energy increased more than that of the van der Waals interaction, corresponding to the dominant role of hydrogen bonding in the vertical model.
    These comprehensive analyses showed that in Type II CNCs, both Coulomb and van der Waals interactions contributed significantly to the strain energy.
    }
    \label{fig:cellulose_nanocrystal_ii_stretch_hydrogen_bond_number_and_energy}
\end{figure}

\clearpage

\subsection*{Stretch transitions of cellulose nanocrystals Type II larger model}\indent
\addcontentsline{toc}{subsection}{\protect\numberline{}Stretch transitions of cellulose nanocrystals Type II larger model}\indent

Among all the models of both the Type I and Type II CNCs, the slant model of Type II is unique because of its two typical fracture behaviors, as proven by the morphologies and stress-strain collection curves.
To further validate these two typical behaviors, a larger slant model of the Type II (composed of 160 cellulose chains with doubled length and width) was constructed and stretched (Figure \ref{fig:cellulose_nanocrystal_ii_larger_stretch_transitions}).
The brittle behavior and restructuring were also reproduced in larger slant models; thus these behaviors are not closely dependent on size or artificial.

\begin{figure}[htbp]
    \centering
    \begin{subfigure}[b]{0.44\textwidth}
        \centering
        \includegraphics[width=0.24\textwidth]{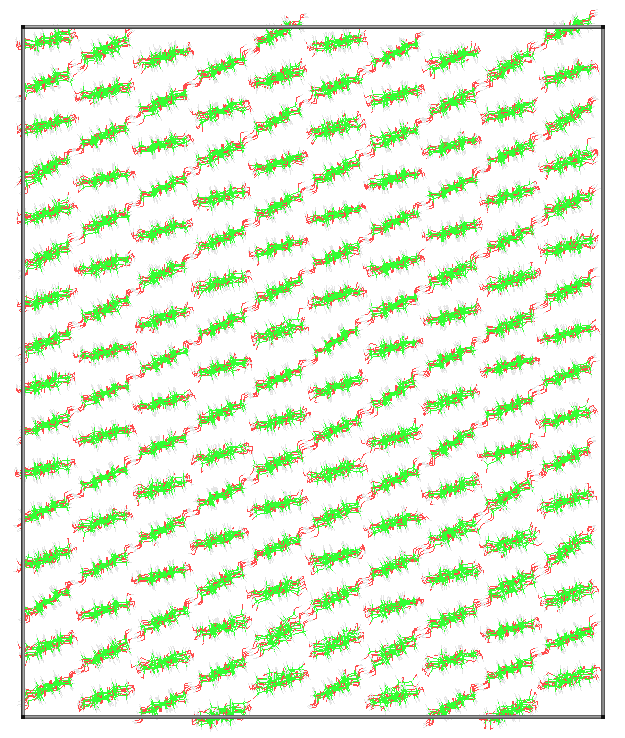}
        \includegraphics[width=0.24\textwidth]{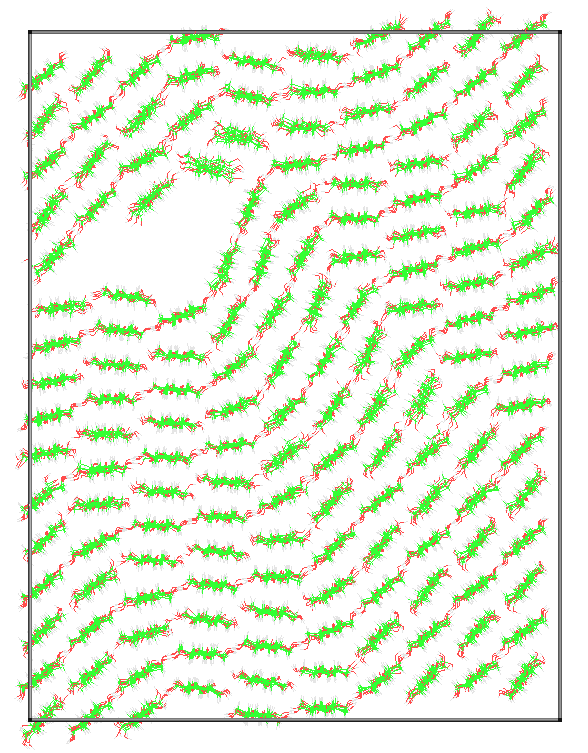}
        \includegraphics[width=0.24\textwidth]{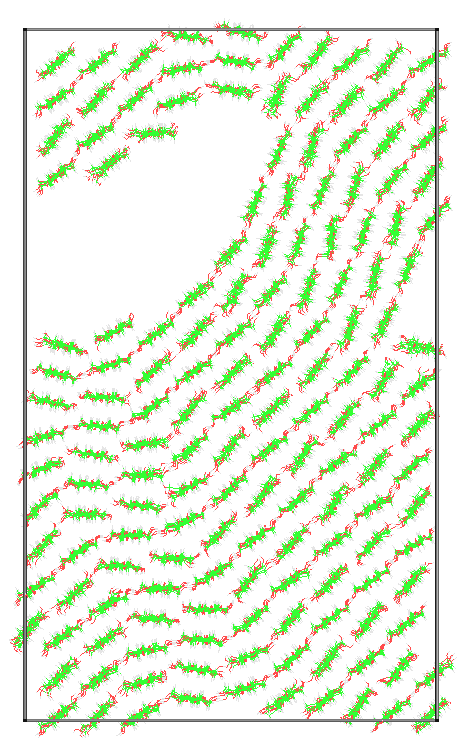}
        \includegraphics[width=0.24\textwidth]{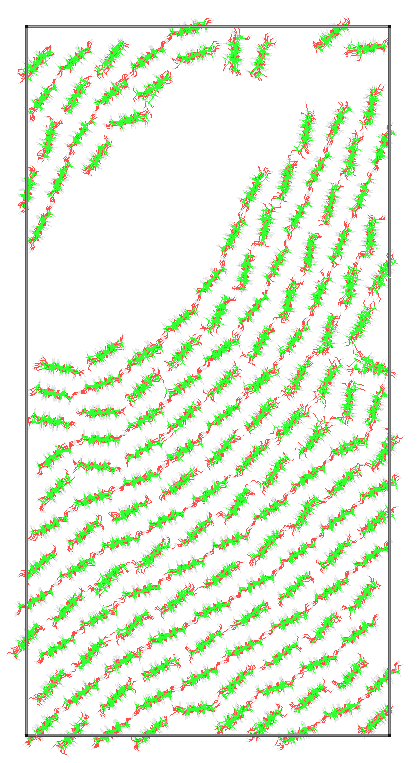}
        \subcaption{}
    \end{subfigure}
    \hspace{0.10\textwidth}
    \begin{subfigure}[b]{0.44\textwidth}
        \centering
        \includegraphics[width=0.24\textwidth]{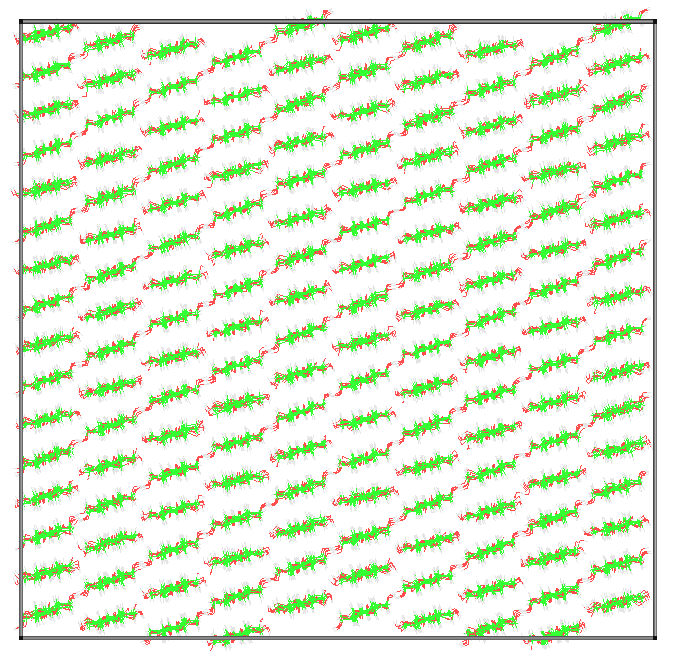}
        \includegraphics[width=0.24\textwidth]{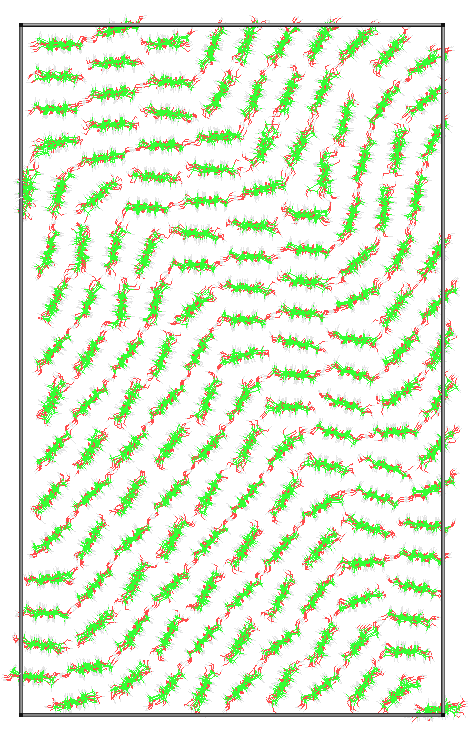}
        \includegraphics[width=0.24\textwidth]{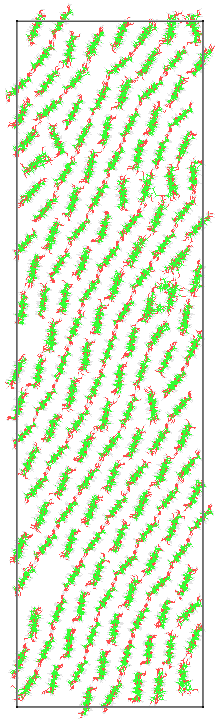}
        \includegraphics[width=0.24\textwidth]{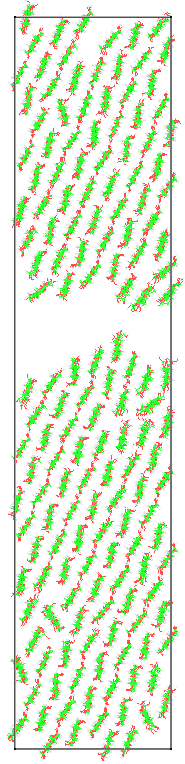}
        \subcaption{}
    \end{subfigure}
    \captionsetup{font=scriptsize}
    \caption{
    Structural transitions of the Type II CNCs larger model during stretching.
    (a) (b) Key frames of the larger slant models from two typical fracture behaviors.
    In contrast to the stable inter layer frictional sliding behavior of Type I, the slant model of Type II may undergo brittle fractures or restructure into a laminar arrangement similar to Type I.
    The restructuring induced by mechanical loads with higher toughness corresponded to an overall friction and rotation, rather than localized fractures.
    Considering the uniqueness of these behaviors, larger models were further simulated and validated.
    These results confirmed that the two typical behaviors are not heavily artificial or size-dependent.
    }
    \label{fig:cellulose_nanocrystal_ii_larger_stretch_transitions}
\end{figure}

\clearpage

\subsection*{Transverse arrangement patterns fractures of the Type I with more unit blocks}\indent
\addcontentsline{toc}{subsection}{\protect\numberline{}Transverse arrangement patterns fractures of the Type I with more unit blocks}\indent

Utilizing the anisotropy and size dependency, the symmetric and cross patterns proved to be effective for toughening.
By doubling the length and width, the models comprising 16 unit blocks arranged in these two patterns were simulated, as shown in Figure \ref{fig:cellulose_nanocrystal_more_transverse_arrangement_fractures}.
These simulation results further demonstrated the toughening mechanisms of the transverse arrangements.

\begin{figure}[htbp]
    \centering
    \scriptsize
    \begin{subfigure}[b]{0.96\textwidth}
        \centering
        \begin{minipage}[b]{0.36\textwidth}
            \centering
            \includegraphics[width=0.24\textwidth]{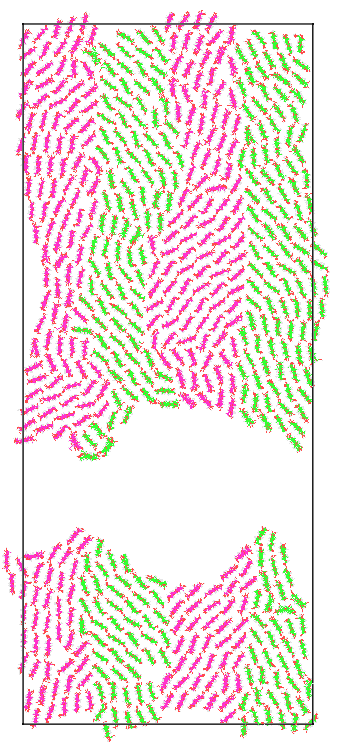}
            \includegraphics[width=0.24\textwidth]{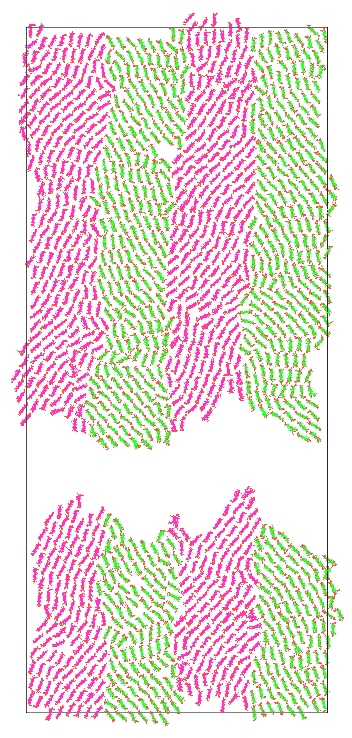}
            \includegraphics[width=0.24\textwidth]{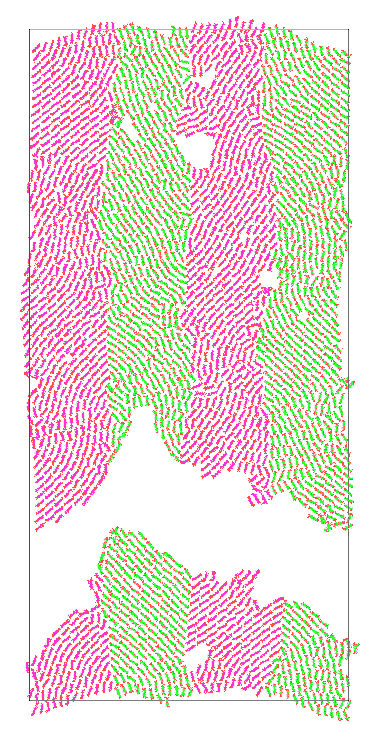}
            \\
            Symmetric
        \end{minipage}
        \hspace{0.12\textwidth}
        \begin{minipage}[b]{0.36\textwidth}
            \centering
            \includegraphics[width=0.24\textwidth]{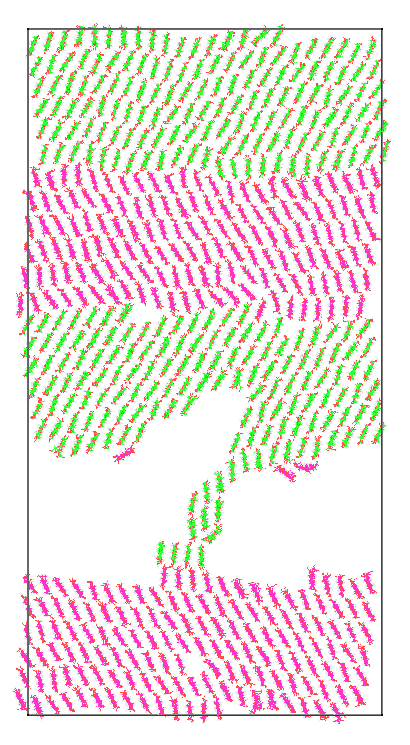}
            \includegraphics[width=0.24\textwidth]{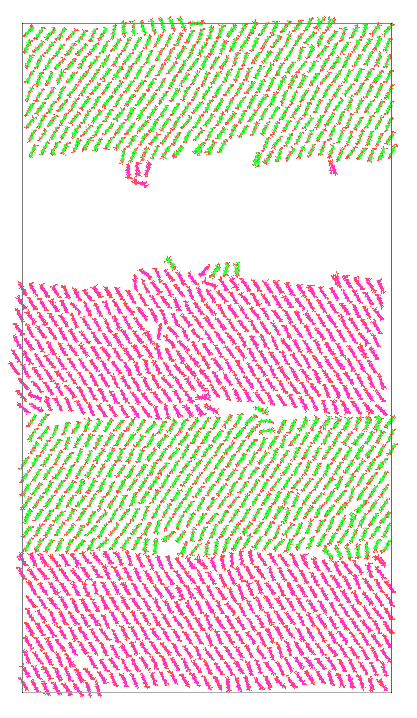}
            \includegraphics[width=0.24\textwidth]{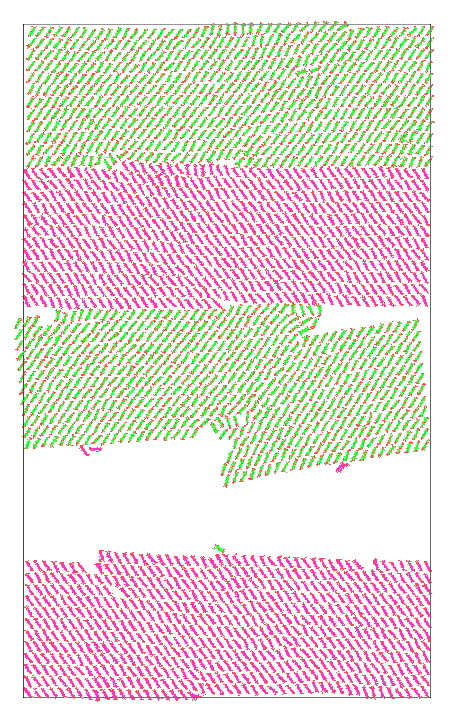}
            \\
            Symmetric Horizontal
        \end{minipage}
        \subcaption{}
    \end{subfigure}
    \\
    \begin{subfigure}[b]{0.96\textwidth}
        \centering
        \begin{minipage}[b]{0.36\textwidth}
            \centering
            \includegraphics[width=0.24\textwidth]{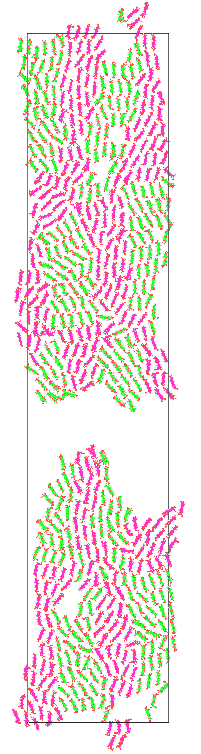}
            \includegraphics[width=0.24\textwidth]{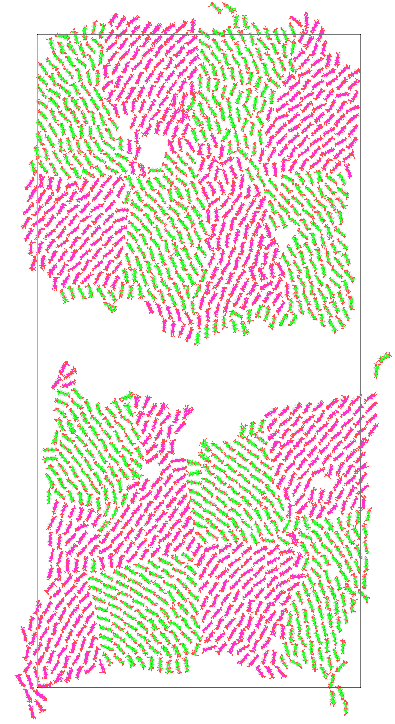}
            \includegraphics[width=0.24\textwidth]{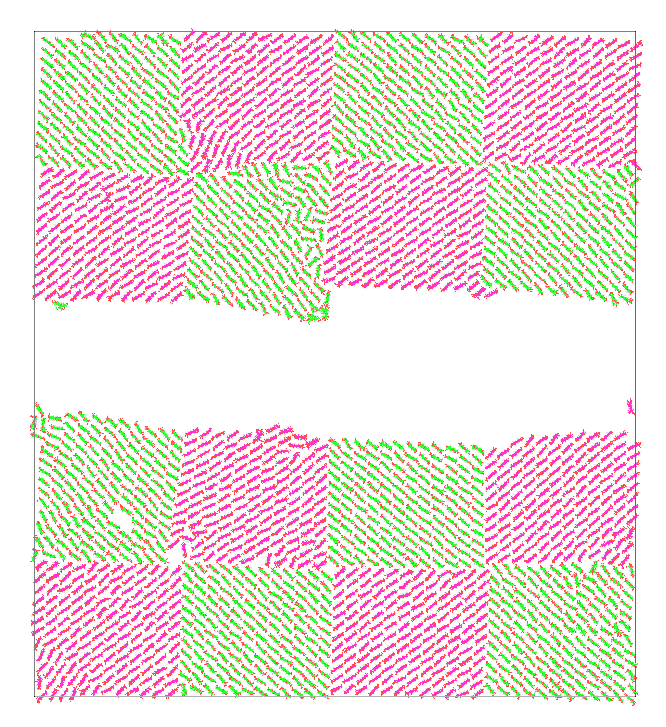}
            \\
            Cross
        \end{minipage}
        \hspace{0.12\textwidth}
        \begin{minipage}[b]{0.36\textwidth}
            \centering
            \includegraphics[width=0.24\textwidth]{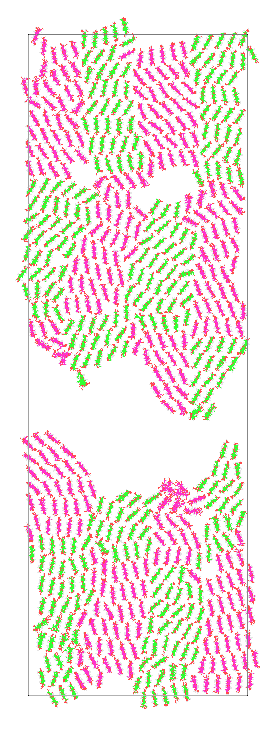}
            \includegraphics[width=0.24\textwidth]{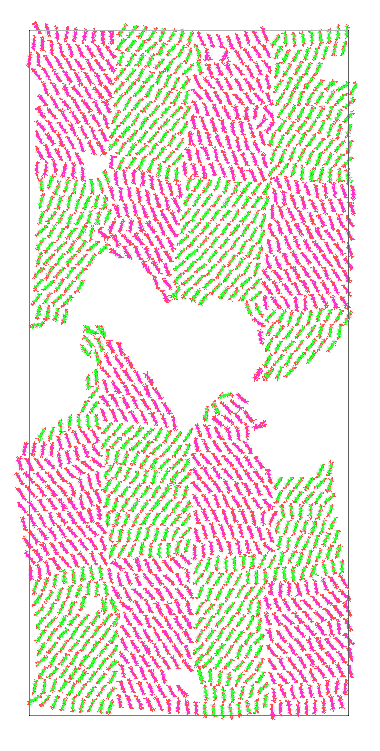}
            \includegraphics[width=0.24\textwidth]{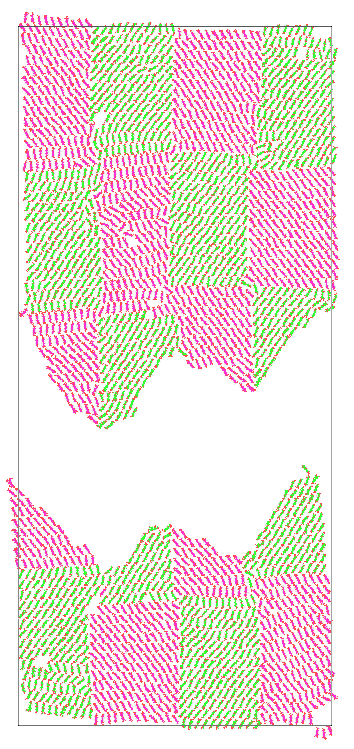}
            \\
            Cross Horizontal
        \end{minipage}
        \subcaption{}
    \end{subfigure}
    \captionsetup{font=scriptsize}
    \caption{
    Transverse arrangement patterns fractures of the Type I CNCs with more unit blocks.
    (a) Fractures of the symmetric arrangements with 16 unit blocks under vertical and horizontal stretching.
    (b) Fractures of the cross arrangements with 16 unit blocks under vertical and horizontal stretching.
    The toughening mechanisms of the transverse patterns and the dependency of the small unit block size were further represented by models composed of 16 unit blocks.
    }
    \label{fig:cellulose_nanocrystal_more_transverse_arrangement_fractures}
\end{figure}

\clearpage

\subsection*{Simulations of different size models and size dependency of cellulose nanocrystals Type II}\indent
\addcontentsline{toc}{subsection}{\protect\numberline{}Simulations of different size models and size dependency of cellulose nanocrystals Type II}\indent

The size dependency of the Type II CNCs was also examined by simulations of different size models.
The aspect ratio of the row number to the column number was 1.6:1, such as 8$\times$5 and 16$\times$10, and the considered lengths were 8, 16, 24, 32, 40, 56, and 80 (Figure \ref{fig:cellulose_nanocrystal_ii_size_dependency}).
By comparing the fractures and data of the models, it was found that the ductility (fracture strain), strength, toughness, and direction angles exhibited a monotonic tendency to decrease with increasing crystal size.

\begin{figure}[htbp]
    \centering
    \begin{subfigure}[b]{0.96\textwidth}
        \centering
        \includegraphics[width=0.12\textwidth]{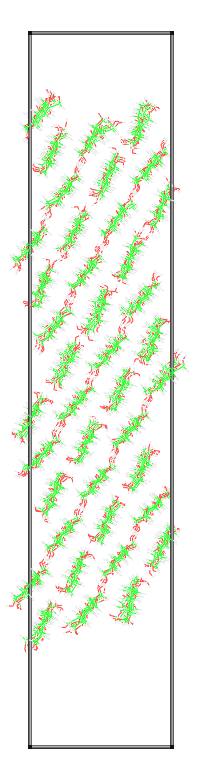}
        \includegraphics[width=0.12\textwidth]{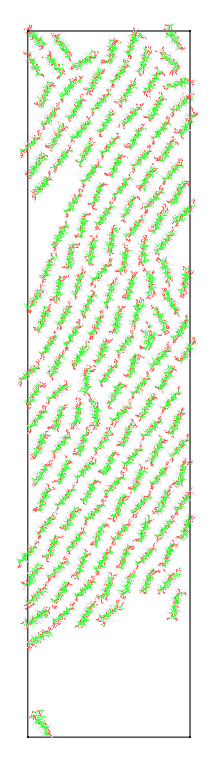}
        \includegraphics[width=0.12\textwidth]{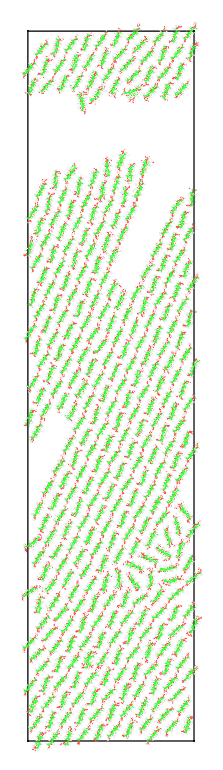}
        \includegraphics[width=0.12\textwidth]{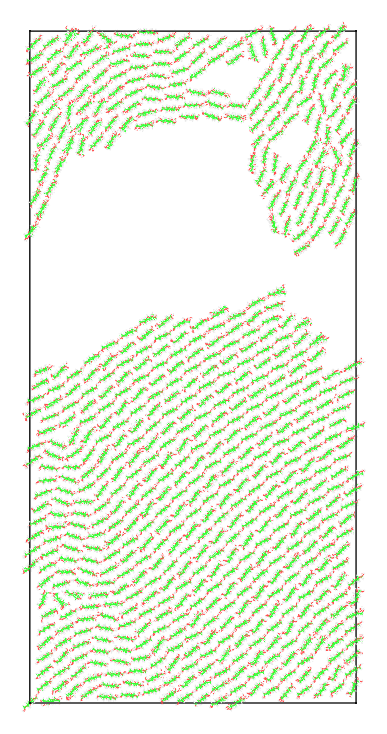}
        \includegraphics[width=0.12\textwidth]{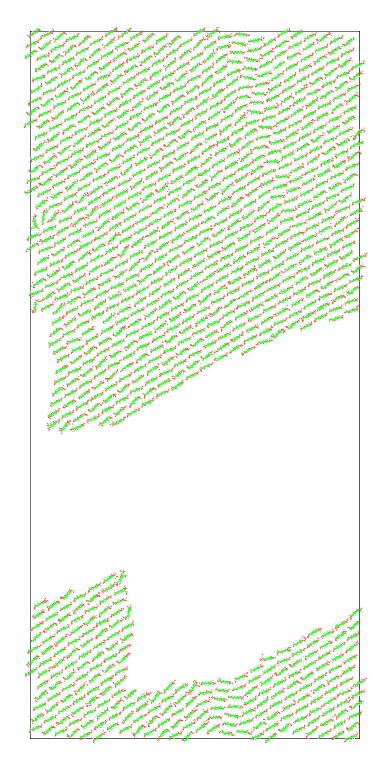}
        \includegraphics[width=0.12\textwidth]{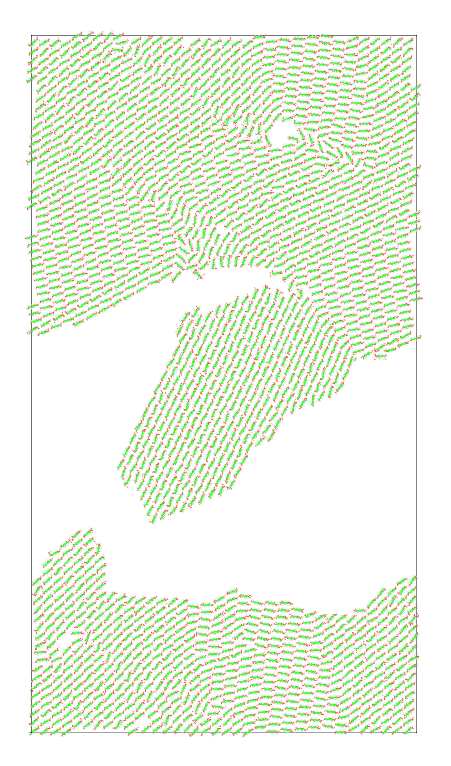}
        \includegraphics[width=0.12\textwidth]{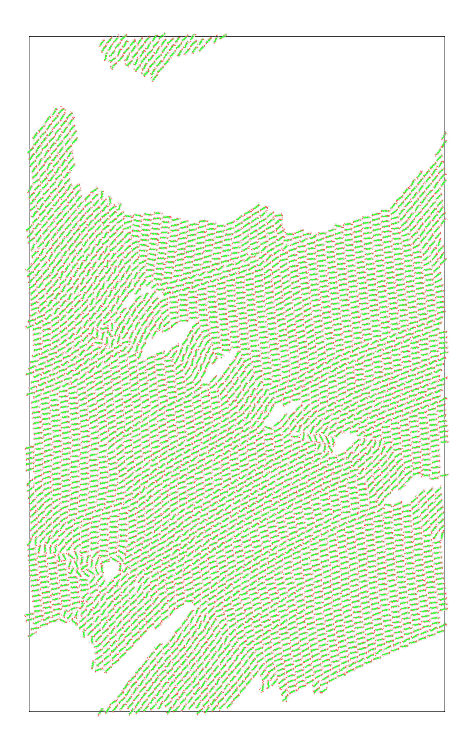}
        \subcaption{}
    \end{subfigure}
    \\
    \begin{subfigure}[b]{0.96\textwidth}
        \centering
        \begin{minipage}[b]{0.32\textwidth}
            \centering
            \includegraphics[width=0.96\textwidth]{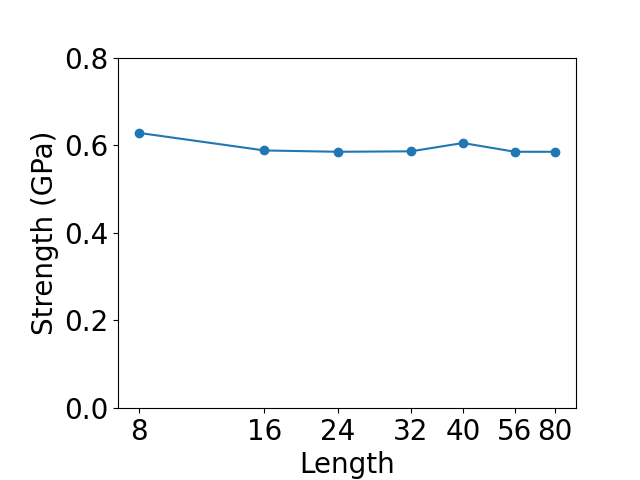}
        \end{minipage}
        \begin{minipage}[b]{0.32\textwidth}
            \centering
            \includegraphics[width=0.96\textwidth]{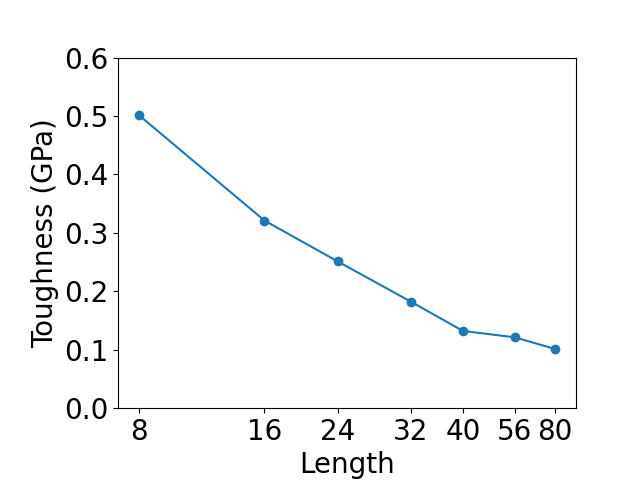}
        \end{minipage}
        \begin{minipage}[b]{0.32\textwidth}
            \centering
            \includegraphics[width=0.96\textwidth]{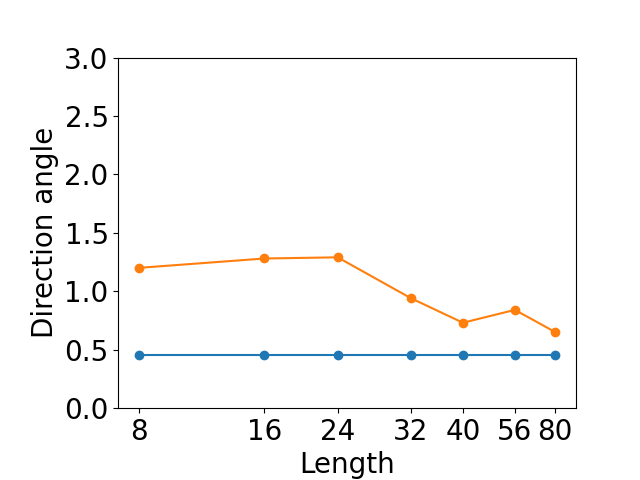}
        \end{minipage}
        \subcaption{}
    \end{subfigure}
    \captionsetup{font=scriptsize}
    \caption{
    Fractures and performances of the Type II CNCs with size.
    (a) Fractures of different sizes.
    The models considered here are Type II CNCs with different rows and columns (the aspect ratio of the row number to column number is 1.6:1), such as 8$\times$5 and 16$\times$10.
    8, 16, 24, 32, 40, 56, and 80 were the considered lengths.
    From the perspective of fracture strain, it can be directly observed that the ductility tended to decrease as the nanocrystal size increased.
    (b) Strength, toughness and direction angles with respect to size.
    As the nanocrystal size increased, the strength, toughness, and direction angle decreased.
    }
    \label{fig:cellulose_nanocrystal_ii_size_dependency}
\end{figure}

\clearpage

The size dependency of the Type II CNCs can also be quantitatively explained by the delta potential energy density, as shown in Figure \ref{fig:cellulose_nanocrystal_ii_delta_energy_density_with_size}.
The delta potential energy density was defined as the ratio of the delta potential energy to the volume of nanocrystals before stretching.
With increasing size, the absolute value of the delta potential energy density gradually decreased and the structures were weaker in resisting stretches.
This could also be explained from the morphological perspective, as the overall volume of varied with the length at the second order, whereas the fractured interface area only increased at a lower order (approximately linearly).

\begin{figure}[htbp]
    \centering
    \begin{subfigure}[b]{0.48\textwidth}
        \includegraphics[width=0.96\textwidth]{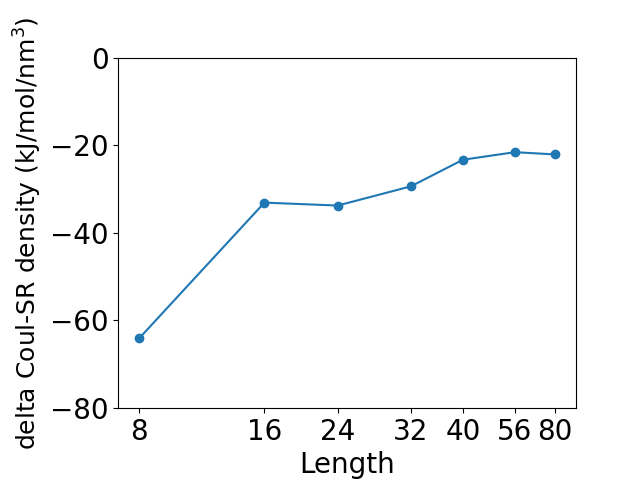}
        \subcaption{}
    \end{subfigure}
    \begin{subfigure}[b]{0.48\textwidth}
        \includegraphics[width=0.96\textwidth]{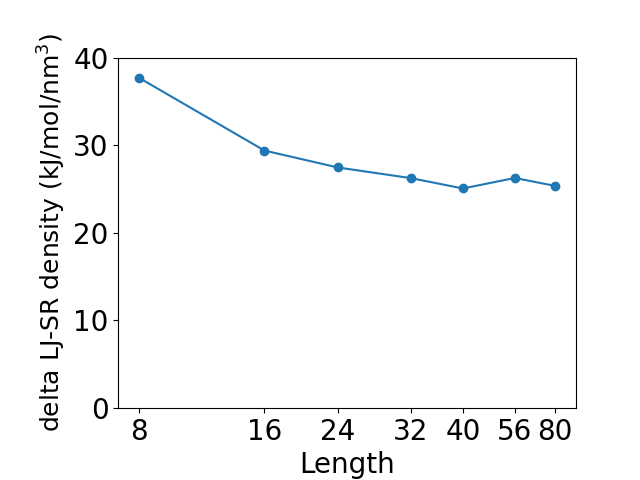}
        \subcaption{}
    \end{subfigure}
    \captionsetup{font=scriptsize}
    \caption{
    Delta potential energy density of the Type II CNCs with size.
    (a) Delta Coulomb potential energy density and (b) delta van der Waals potential energy density with size.
    The delta potential energy density was defined as the ratio of the delta potential energy during stretching relative to the nanocrystal volume before stretching, that is, the delta potential energy per unit volume.
    As the size of the nanocrystal increased, the absolute value of the delta potential energy density during stretching gradually decreased, particularly for the van der Waals interaction resisting stretches.
    From the perspective of structure, larger nanocrystals have a stronger ability to maintain themselves.
    Even though restructuring was observed in all the models, in larger nanocrystals, the parts away from the fracture interface can maintain a structure similar to that of the crystal.
    The structural changes were not significant compared with those in the smallest 8$\times$5 model.
    Based on the delta potential energy density, the damage to the CNCs is a localized interaction at the fracture interface, therefore the delta potential energy density does not increase linearly with the crystal volume.
    The volume of the nanocrystal increased quadratically with the length, whereas the delta potential energy of the fracture interface increased at a lower power.
    Therefore, the delta potential energy density and mechanical performance of the Type II CNCs weakened as the nanocrystal size increased.
    }
    \label{fig:cellulose_nanocrystal_ii_delta_energy_density_with_size}
\end{figure}

\clearpage

\subsection*{Transverse arrangement patterns of the Type II}\indent
\addcontentsline{toc}{subsection}{\protect\numberline{}Transverse arrangement fractures of the Type II}\indent

Considering the anisotropy and size dependency of the Type II CNCs, symmetric and cross pattern models were also constructed and simulated, as shown in Figure \ref{fig:cellulose_nanocrystal_ii_transverse_arrangement_fractures}.
The cross pattern represents a biaxial permutation of the symmetric arrangement.
To form a model, 4 unit blocks were arranged, where unit block size included 8$\times$5, 12$\times$7, and 16$\times$10 rows and columns.
As shown in the figures, only the symmetric patten under vertical stretching exhibited high ductility and strength.
The weak interfaces in the symmetric pattern under horizontal stretching and the cross pattern under both loads, further confirmed the performance dependency of the crystal structures and the periodicity of Type II.
For the symmetric pattern under vertical stretching, it is evident that the ductility and toughness depend on the size of the unit blocks.

\begin{figure}[htbp]
    \centering
    \scriptsize
    \begin{subfigure}[b]{0.96\textwidth}
        \centering
        \begin{minipage}[b]{0.24\textwidth}
            \centering
            \includegraphics[width=0.96\textwidth]{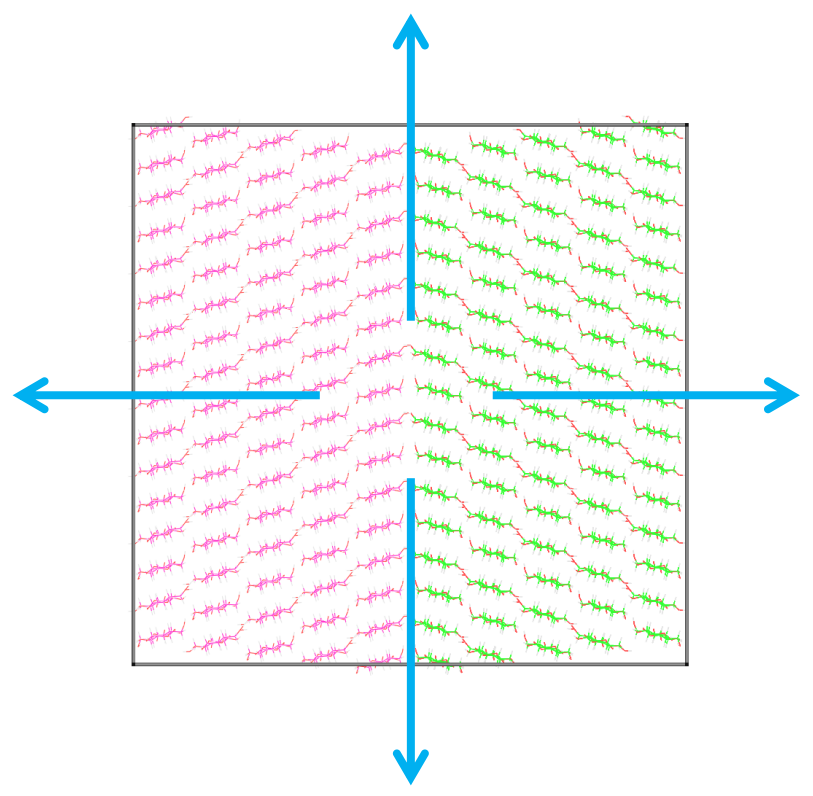}
            \\
            Symmetric
        \end{minipage}
        \begin{minipage}[b]{0.24\textwidth}
            \centering
            \includegraphics[width=0.96\textwidth]{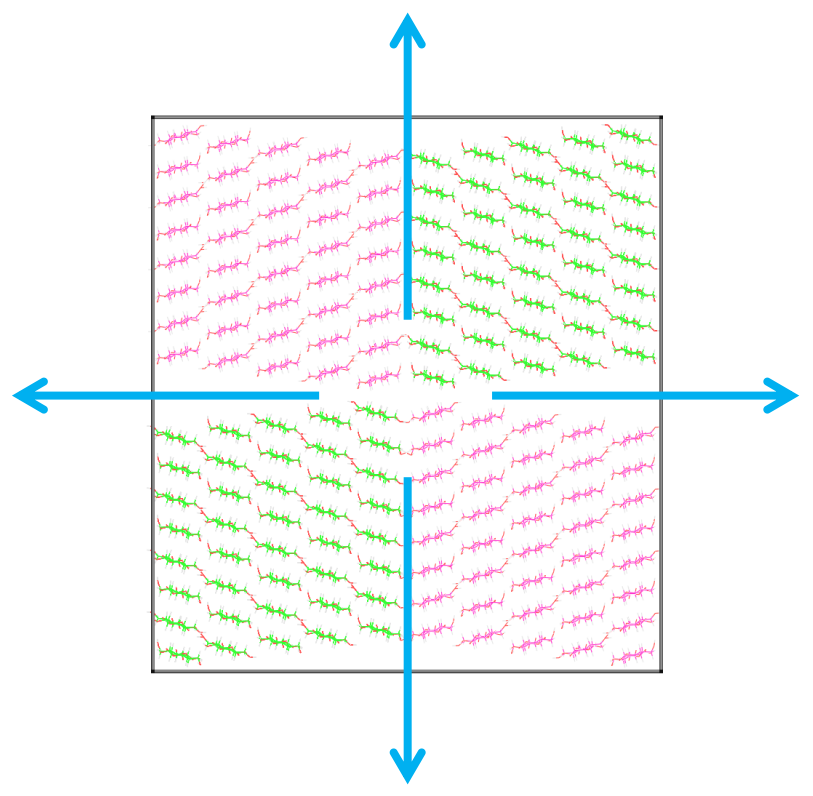}
            \\
            Cross
        \end{minipage}
        \subcaption{}
    \end{subfigure}
    \\
    \begin{subfigure}[b]{0.96\textwidth}
        \centering
        \begin{minipage}[b]{0.36\textwidth}
            \centering
            \includegraphics[width=0.24\textwidth]{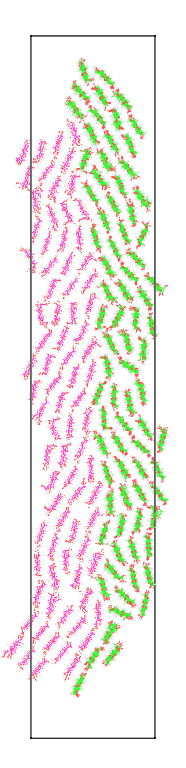}
            \includegraphics[width=0.24\textwidth]{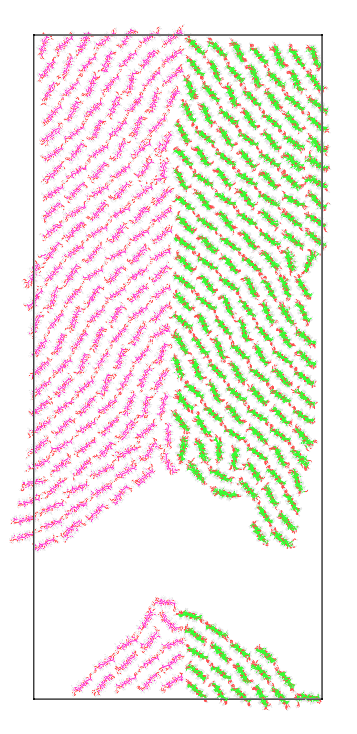}
            \includegraphics[width=0.24\textwidth]{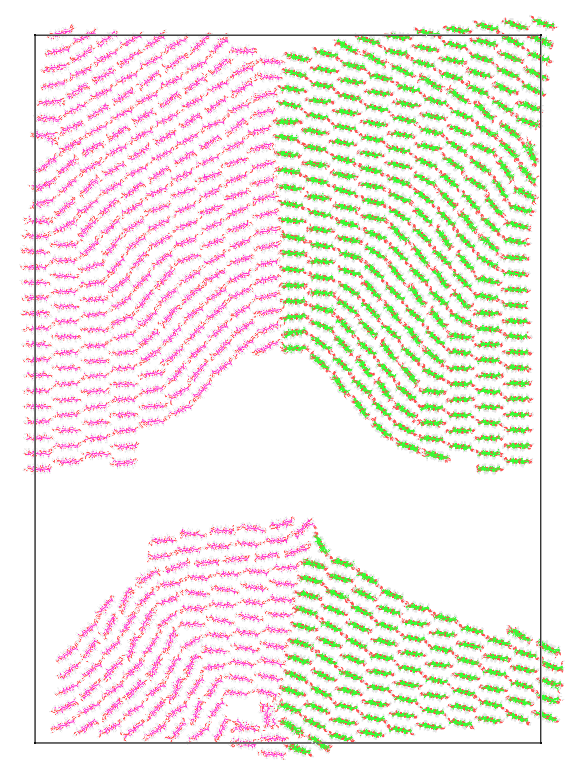}
            \\
            Symmetric
        \end{minipage}
        \hspace{0.12\textwidth}
        \begin{minipage}[b]{0.36\textwidth}
            \centering
            \includegraphics[width=0.24\textwidth]{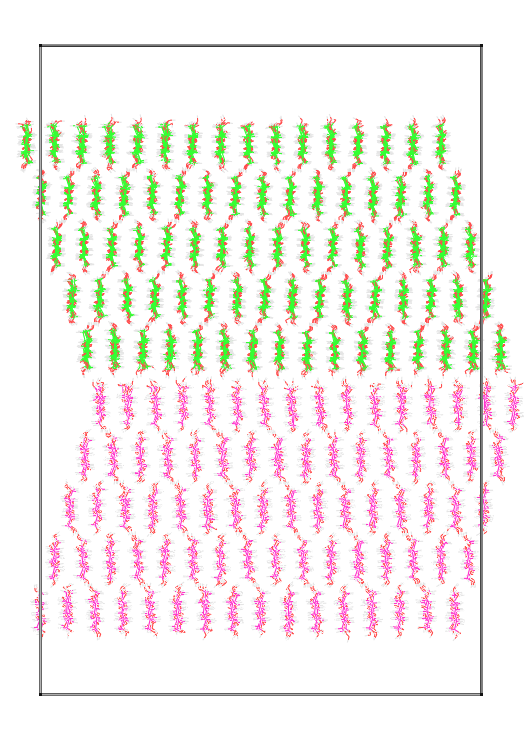}
            \includegraphics[width=0.24\textwidth]{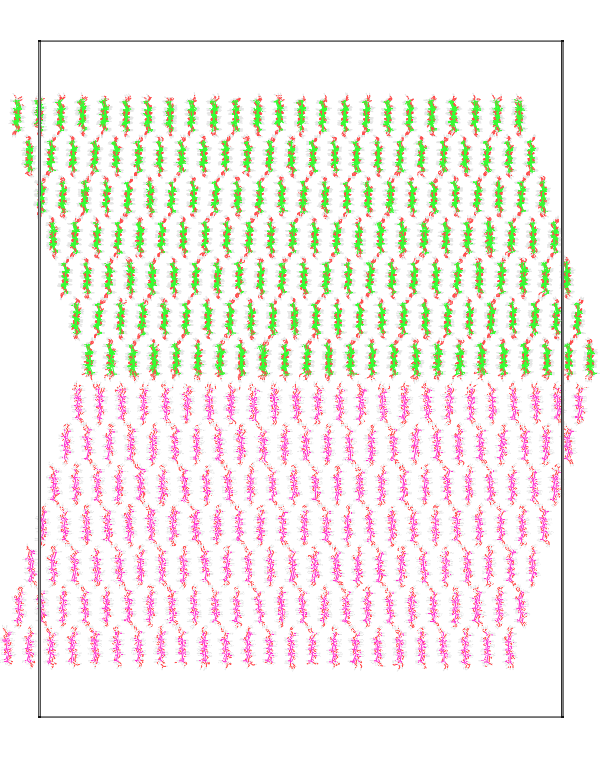}
            \includegraphics[width=0.24\textwidth]{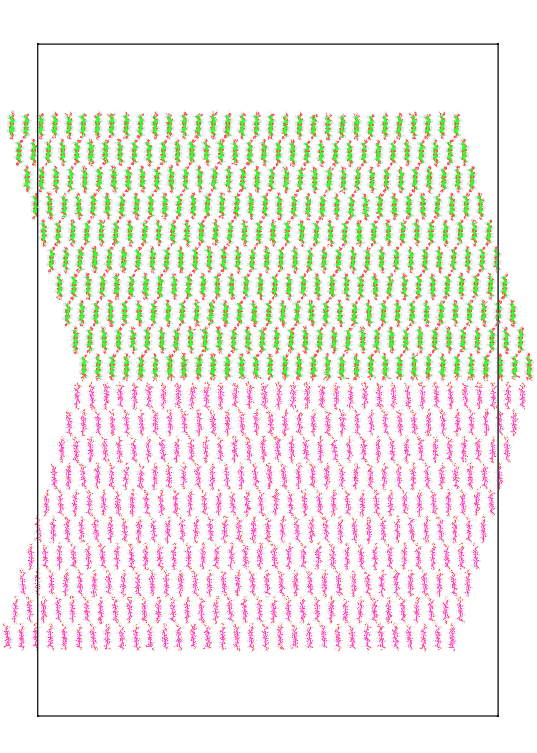}
            \\
            Symmetric Horizontal
        \end{minipage}
        \subcaption{}
    \end{subfigure}
    \\
    \begin{subfigure}[b]{0.96\textwidth}
        \centering
        \begin{minipage}[b]{0.36\textwidth}
            \centering
            \includegraphics[width=0.24\textwidth]{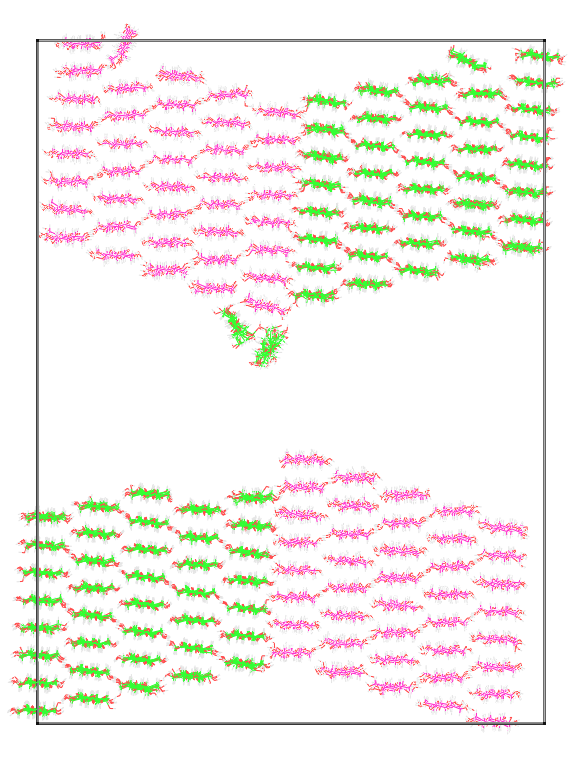}
            \includegraphics[width=0.24\textwidth]{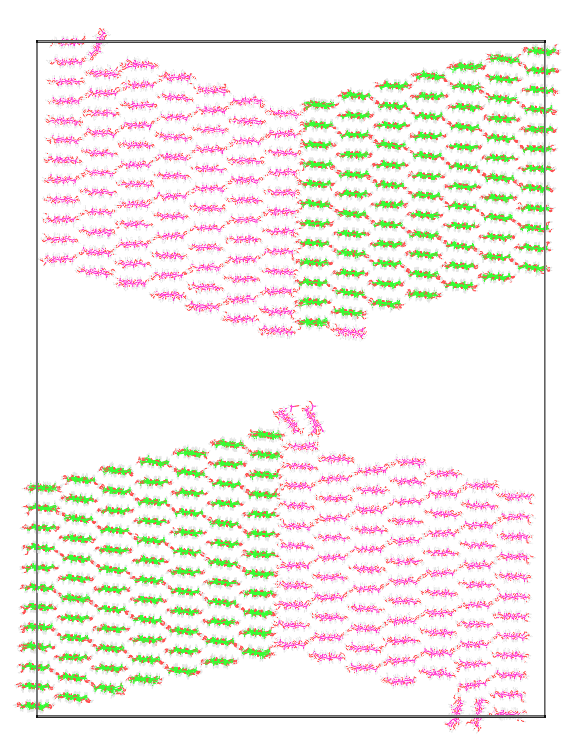}
            \includegraphics[width=0.24\textwidth]{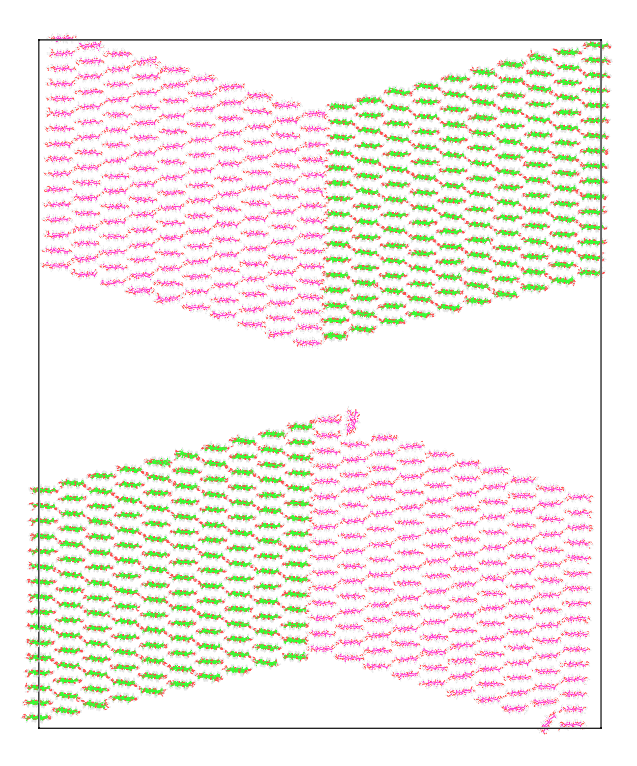}
            \\
            Cross
        \end{minipage}
        \hspace{0.12\textwidth}
        \begin{minipage}[b]{0.36\textwidth}
            \centering
            \includegraphics[width=0.24\textwidth]{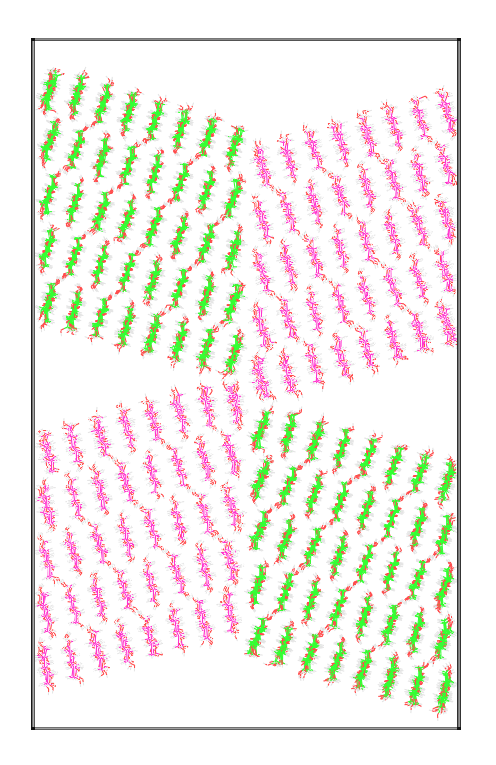}
            \includegraphics[width=0.24\textwidth]{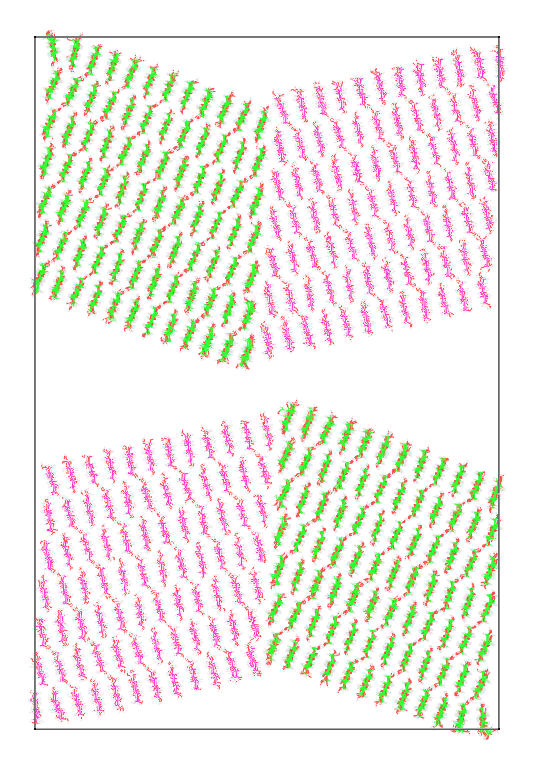}
            \includegraphics[width=0.24\textwidth]{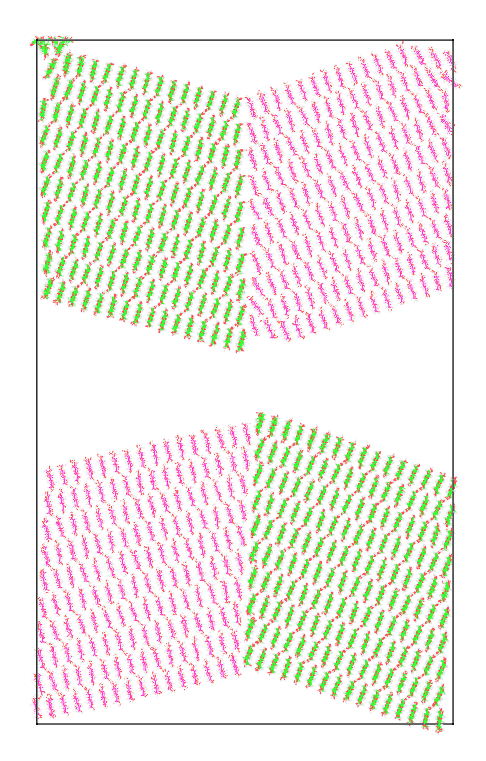}
            \\
            Cross Horizontal
        \end{minipage}
        \subcaption{}
    \end{subfigure}
    \captionsetup{font=scriptsize}
    \caption{
    Transverse arrangement patterns and corresponding fractures of the Type II CNCs.
    (a) Two transverse arrangement patterns: symmetric and cross.
    The cross pattern represents a biaxial permutation of the symmetric arrangement.
    Based on the structure, the performances of the two arrangement patterns differed in the vertical and horizontal directions, and the models were stretched in both directions.
    The structures stretched under horizontal loads were rotated counter clockwise, including models composed of different unit block sizes (8$\times$5, 12$\times$7, and 16$\times$10 rows and columns; one model was composed of 4 of unit blocks).
    (b) Fractures of the symmetric arrangements under vertical and horizontal stretching.
    The symmetric arrangements exhibited good toughness and ductility under vertical loading but were weak when subjected to horizontal loading, owing to the weak interfaces.
    (c) Fractures of the cross arrangements under vertical and horizontal stretching.
    The cross arrangements did not exhibit good toughness and ductility under either vertical or horizontal loading, emphasizing the configuration differences between Type I and Type II.
    The Type II CNCs relied on the ideal crystal structure and periodicity to exhibit good mechanical properties.
    Only in the symmetric arrangements under vertical stretching, the frictions and restructuring were hindered and led to localized rotation becoming the dominant deformation mechanism, which resulted in improved toughness and ductility.
    Additionally, these arrangements were affected by the size dependency of the units.
    The structures composed of smaller units exhibited better toughness and ductility.
    }
    \label{fig:cellulose_nanocrystal_ii_transverse_arrangement_fractures}
\end{figure}

\clearpage

By doubling the length and width, the models comprising 16 unit blocks arranged in these two patterns were simulated, as shown in Figure \ref{fig:cellulose_nanocrystal_ii_more_transverse_arrangement_fractures}.
These simulation results further demonstrated the toughening mechanism of the symmetric pattern under vertical stretching.

\begin{figure}[htbp]
    \centering
    \scriptsize
    \begin{subfigure}[b]{0.96\textwidth}
        \centering
        \begin{minipage}[b]{0.36\textwidth}
            \centering
            \includegraphics[width=0.24\textwidth]{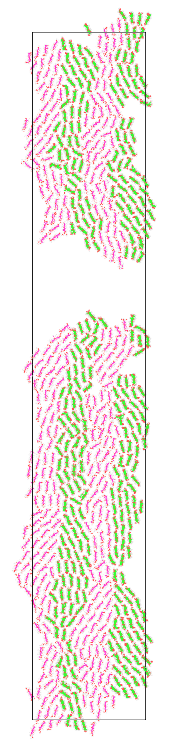}
            \includegraphics[width=0.24\textwidth]{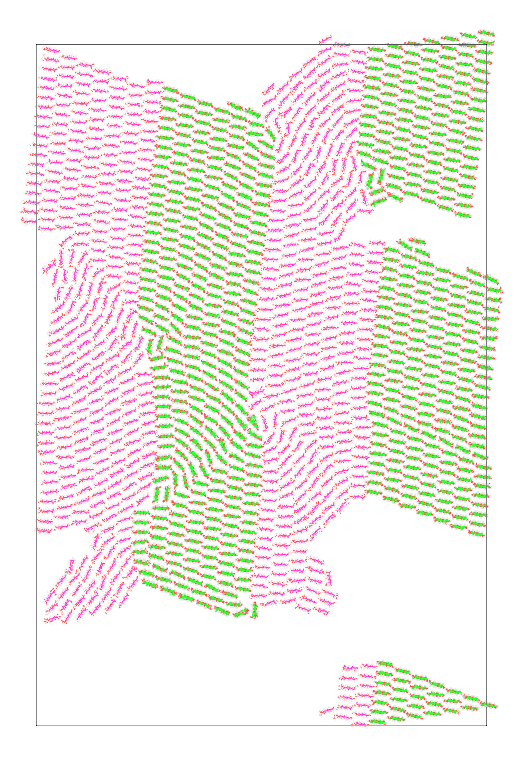}
            \includegraphics[width=0.24\textwidth]{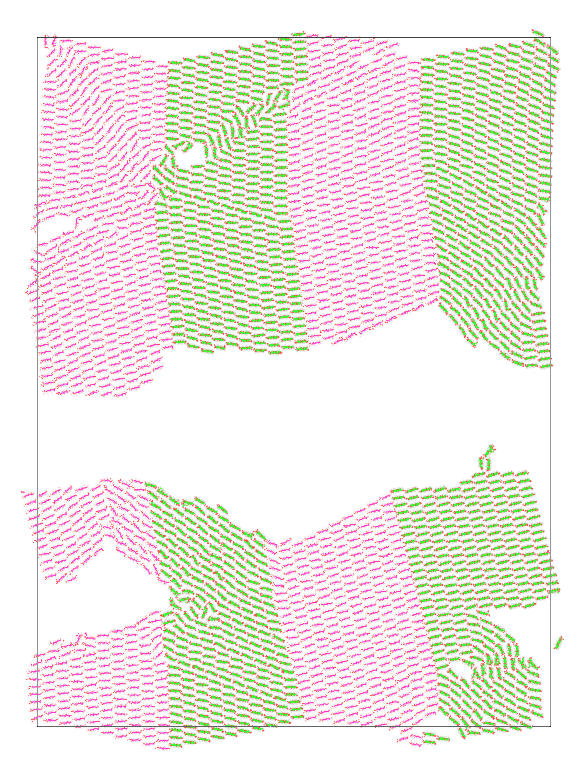}
            \\
            Symmetric
        \end{minipage}
        \hspace{0.12\textwidth}
        \begin{minipage}[b]{0.36\textwidth}
            \centering
            \includegraphics[width=0.24\textwidth]{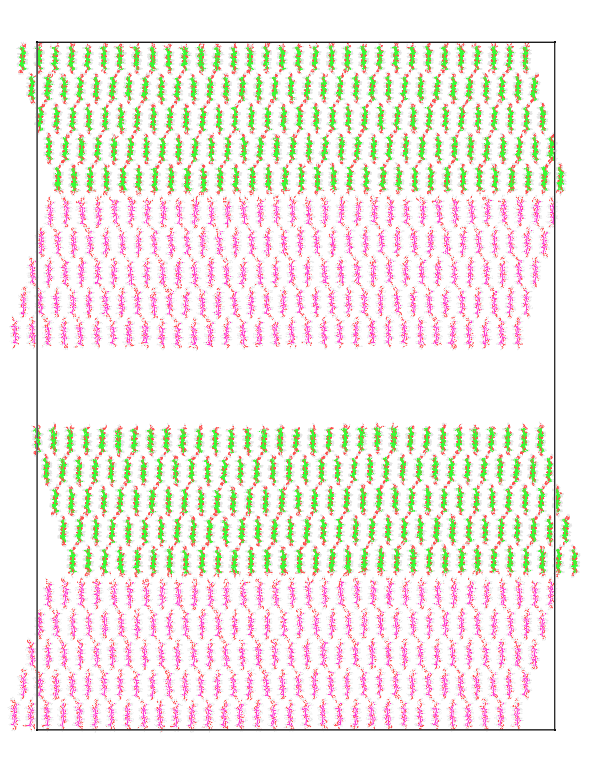}
            \includegraphics[width=0.24\textwidth]{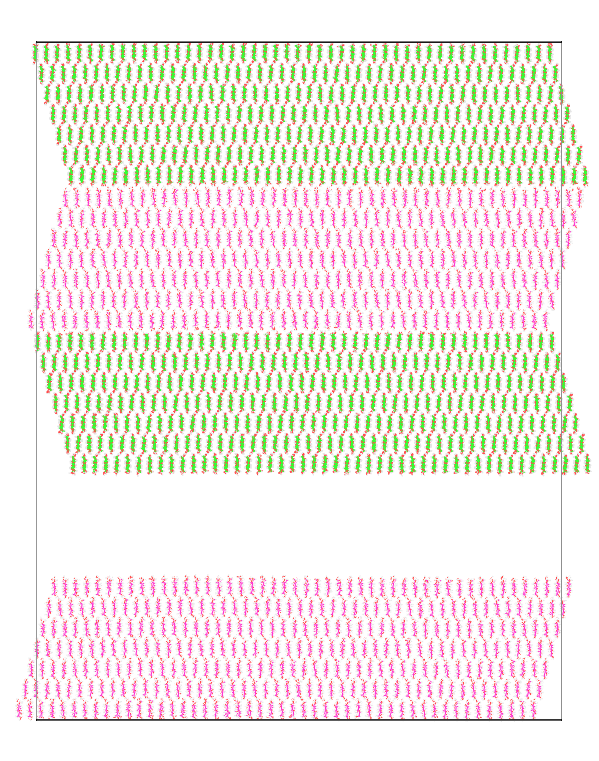}
            \includegraphics[width=0.24\textwidth]{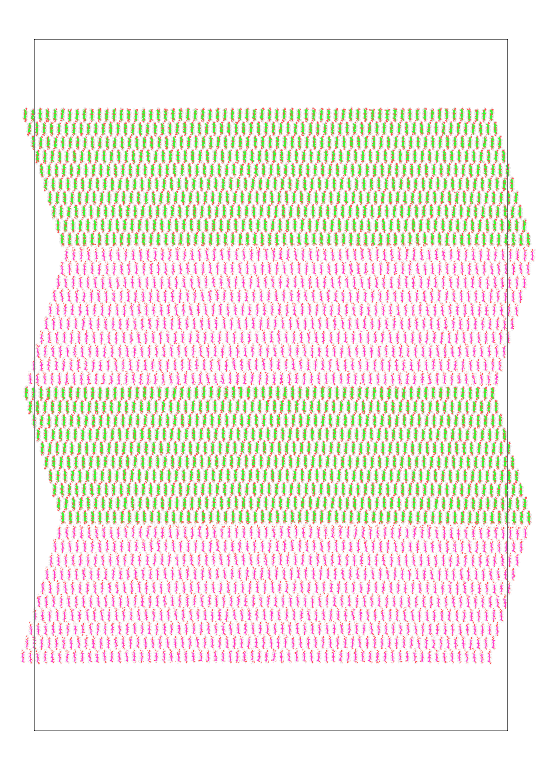}
            \\
            Symmetric Horizontal
        \end{minipage}
        \subcaption{}
    \end{subfigure}
    \\
    \begin{subfigure}[b]{0.96\textwidth}
        \centering
        \begin{minipage}[b]{0.36\textwidth}
            \centering
            \includegraphics[width=0.24\textwidth]{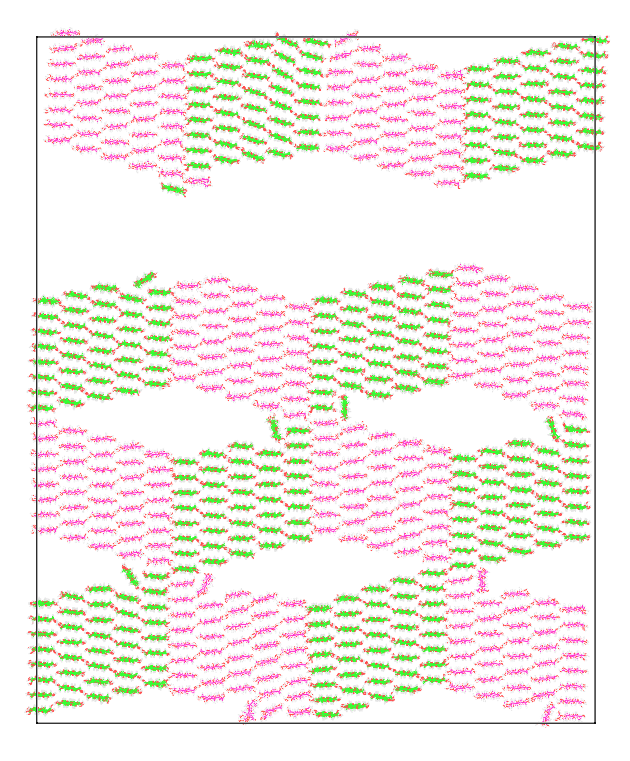}
            \includegraphics[width=0.24\textwidth]{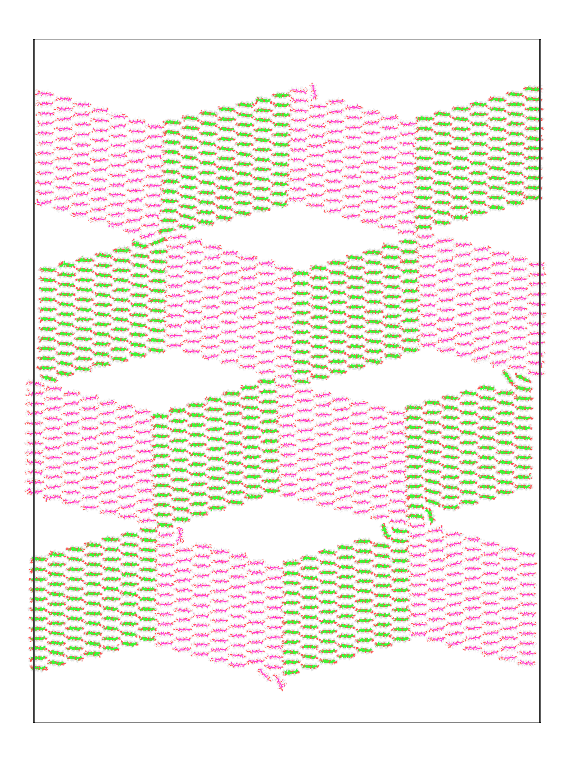}
            \includegraphics[width=0.24\textwidth]{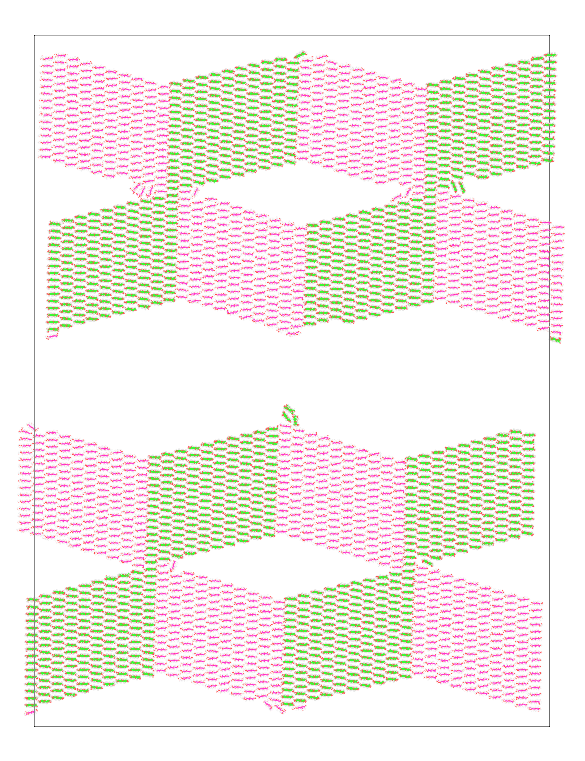}
            \\
            Cross
        \end{minipage}
        \hspace{0.12\textwidth}
        \begin{minipage}[b]{0.36\textwidth}
            \centering
            \includegraphics[width=0.24\textwidth]{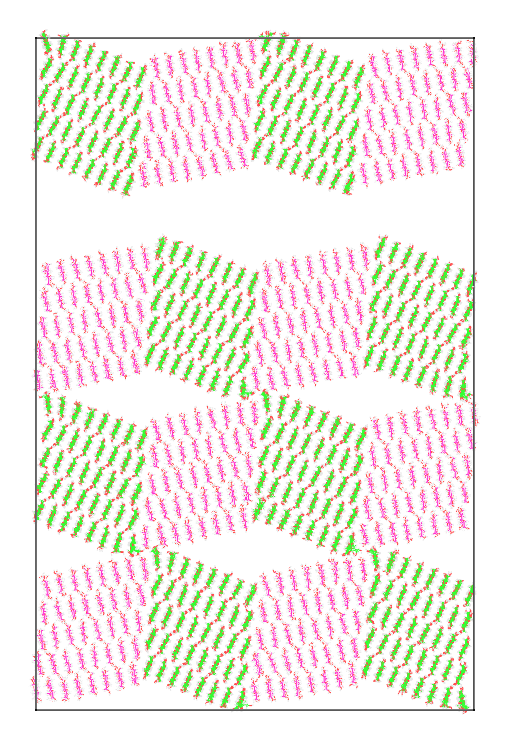}
            \includegraphics[width=0.24\textwidth]{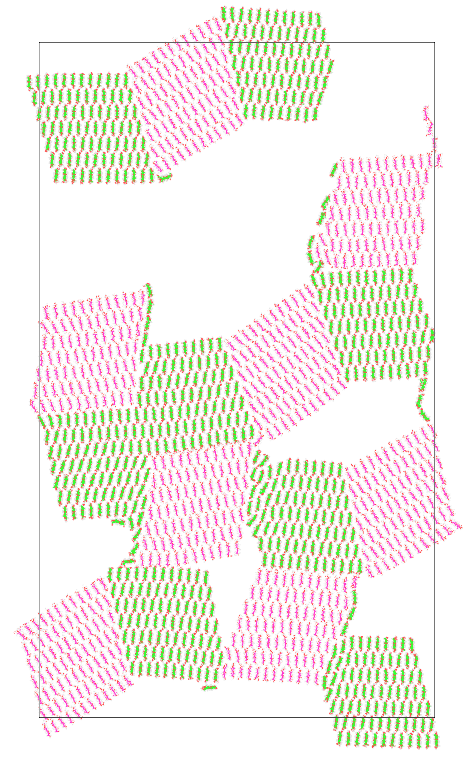}
            \includegraphics[width=0.24\textwidth]{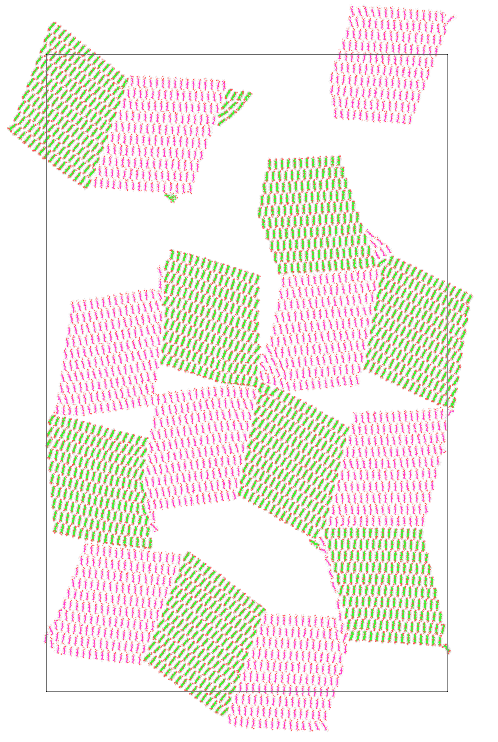}
            \\
            Cross Horizontal
        \end{minipage}
        \subcaption{}
    \end{subfigure}
    \captionsetup{font=scriptsize}
    \caption{
    Transverse arrangement patterns fractures of the Type II CNCs with more unit blocks.
    (a) Fractures of the symmetric arrangements with 16 unit blocks under vertical and horizontal stretching.
    (b) Fractures of the cross arrangements with 16 unit blocks under vertical and horizontal stretching.
    The toughening mechanism of the symmetric pattern and the dependency on small unit block size were further represented by models composed of 16 unit blocks.
    }
    \label{fig:cellulose_nanocrystal_ii_more_transverse_arrangement_fractures}
\end{figure}

\clearpage

The quantitative strength and toughness data are shown in Figure \ref{fig:cellulose_nanocrystal_ii_transverse_arrangement_performance_with_patterns}.
The toughening of the symmetric pattern under vertical stretching and the size dependency of the unit blocks were further emphasized.

\begin{figure}[htbp]
    \centering
    \begin{subfigure}[b]{0.96\textwidth}
        \includegraphics[width=0.48\textwidth]{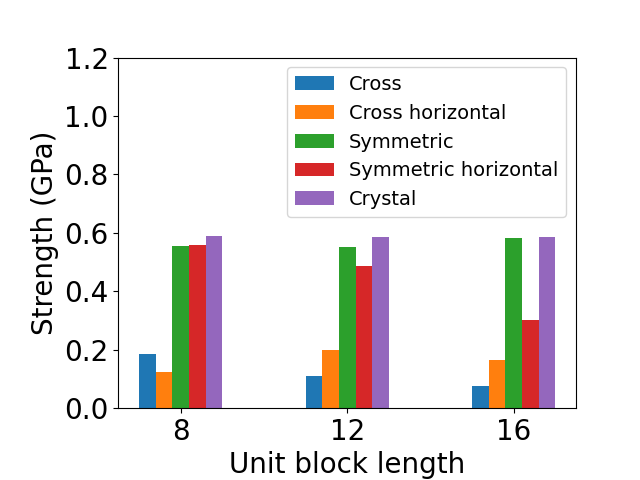}
        \includegraphics[width=0.48\textwidth]{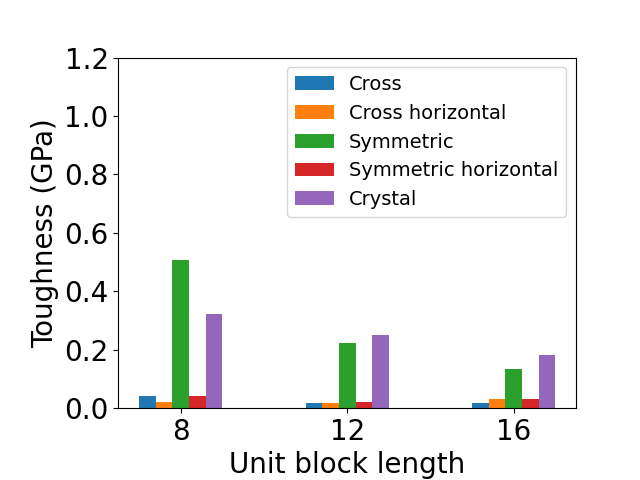}
        \subcaption{}
    \end{subfigure}
    \\
    \begin{subfigure}[b]{0.96\textwidth}
        \includegraphics[width=0.48\textwidth]{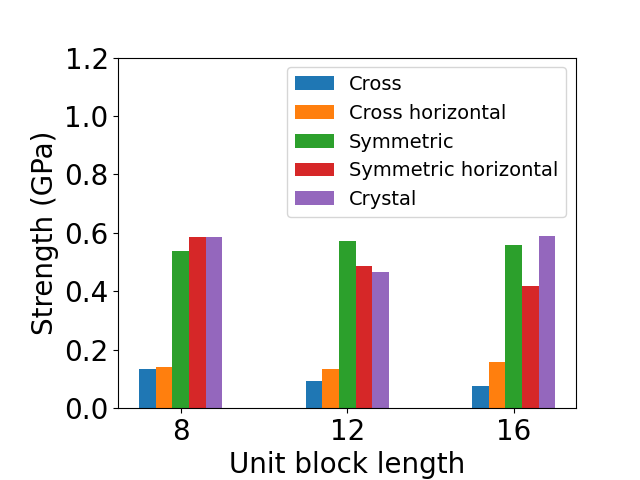}
        \includegraphics[width=0.48\textwidth]{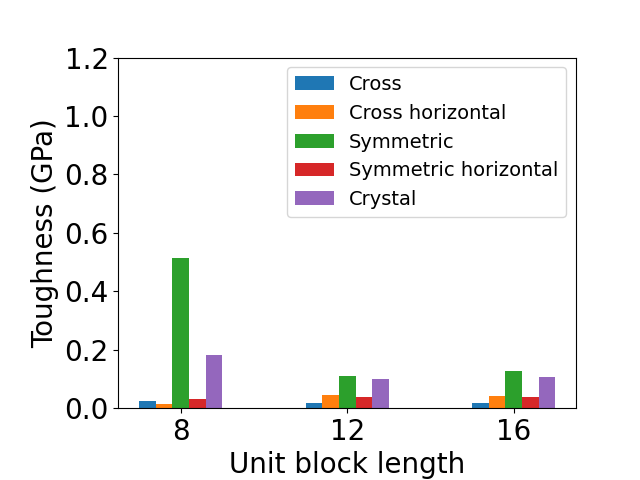}
        \subcaption{}
    \end{subfigure}
    \captionsetup{font=scriptsize}
    \caption{
    Mechanical performance of transverse arrangement patterns of the Type II CNCs.
    (a) Strength and toughness of the transverse patterns.
    (b) Strength and toughness of the transverse patterns with more unit blocks.
    By comparing with crystal models of the same overall dimensions, it is clear that only the symmetric pattern models with vertical stretching can improve the ductility and toughness, which is closely related to the configuration of Type II.
    The toughening mechanism of the symmetric pattern and the dependency on the small unit block size were further represented by models composed of 16 unit blocks.
    }
    \label{fig:cellulose_nanocrystal_ii_transverse_arrangement_performance_with_patterns}
\end{figure}

\end{document}
